# Supplementary material for: Assessment of the Performance of DFT Functionals Using Off-Diagonal Hypervirial Relationships
Source: arXiv:2102.07603 source file (2021-02-15)
Supplement: Supplementary file 1 [file Supp_Mat.pdf]

# Supporting Material

## Assessment of the Performance of DFT Functionals Using Off-Diagonal Hypervirial Relationships

*F. F. Summa<sup>1</sup>, G. Monaco<sup>1</sup>, P. Lazzeretti<sup>2</sup>, R. Zanasi<sup>1</sup>*

<sup>1</sup> Dipartimento di Chimica e Biologia “A. Zambelli”,  
Università degli studi di Salerno, via Giovanni Paolo II 132,  
Fisciano 84084, SA, Italy

<sup>2</sup> Istituto di Struttura della Materia,  
CNR, via del Fosso del Cavaliere 100,  
00133 Roma, Italy

### Contents

|          |                                                                |            |
|----------|----------------------------------------------------------------|------------|
| <b>1</b> | <b>Cartesian coordinates in Bohr used for the calculations</b> | <b>S2</b>  |
| <b>2</b> | <b>Disaggregated data</b>                                      | <b>S22</b> |

# 1 Cartesian coordinates in Bohr used for the calculations

Table S1: Geometries used for the APFD calculations.

| C <sub>2</sub> H <sub>6</sub>   |          |          |          | H <sub>2</sub> O <sub>2</sub> |          |          |          |
|---------------------------------|----------|----------|----------|-------------------------------|----------|----------|----------|
| C                               | 0.00000  | 1.44480  | -0.00588 | O                             | -0.01493 | 1.34871  | -0.28924 |
| C                               | 0.00000  | -1.44480 | -0.00588 | O                             | 0.01493  | -1.34871 | -0.28924 |
| H                               | 1.35400  | 2.20973  | -1.35990 | H                             | -1.46110 | -1.71931 | 0.70836  |
| H                               | -1.85818 | 2.22113  | -0.44116 | H                             | 1.46110  | 1.71931  | 0.70836  |
| H                               | 0.55582  | 2.18935  | 1.83636  |                               |          |          |          |
| H                               | -1.35400 | -2.20973 | -1.35990 |                               |          |          |          |
| H                               | 1.85818  | -2.22113 | -0.44116 |                               |          |          |          |
| H                               | -0.55582 | -2.18935 | 1.83636  |                               |          |          |          |
| CH <sub>3</sub> NH <sub>2</sub> |          |          |          | N <sub>2</sub> H <sub>4</sub> |          |          |          |
| C                               | 1.33206  | -0.00074 | 0.03163  | N                             | 0.00000  | 1.36465  | -0.20738 |
| H                               | 2.04162  | -0.93385 | 1.73990  | N                             | 0.00000  | -1.36465 | -0.20738 |
| H                               | 2.18833  | -0.96194 | -1.58345 | H                             | -0.95917 | 2.02503  | 1.32681  |
| H                               | 2.03607  | 1.93425  | 0.02265  | H                             | 1.80487  | 1.90909  | 0.12487  |
| N                               | -1.40769 | -0.00177 | -0.21550 | H                             | -1.80487 | -1.90909 | 0.12487  |
| H                               | -2.20688 | -1.55448 | 0.54790  | H                             | 0.95917  | -2.02503 | 1.32681  |
| H                               | -2.19769 | 1.53287  | 0.59169  |                               |          |          |          |
| CH <sub>3</sub> OH              |          |          |          | NH <sub>2</sub> OH            |          |          |          |
| C                               | 1.25003  | 0.03560  | 0.00408  | N                             | 1.30289  | 0.11122  | -0.27029 |
| H                               | 2.04467  | -1.59153 | -0.97783 | O                             | -1.36282 | -0.23038 | 0.10816  |
| H                               | 2.01278  | 0.09007  | 1.92707  | H                             | -2.07337 | 1.34785  | -0.42942 |
| H                               | 1.87463  | 1.73312  | -0.99866 | H                             | 1.99213  | -1.58215 | 0.31331  |
| O                               | -1.40800 | -0.23159 | 0.00267  | H                             | 1.86361  | 1.29876  | 1.14284  |
| H                               | -2.16824 | 1.40747  | 0.00359  |                               |          |          |          |

Table S2: Geometries used for the B3LYP calculations.

| C <sub>2</sub> H <sub>6</sub>   |          |          |          | H <sub>2</sub> O <sub>2</sub> |          |          |          |
|---------------------------------|----------|----------|----------|-------------------------------|----------|----------|----------|
| C                               | 0.00000  | 1.44792  | -0.00580 | O                             | 0.00000  | 1.36782  | -0.10932 |
| C                               | 0.00000  | -1.44792 | -0.00580 | O                             | 0.00000  | -1.36782 | -0.10932 |
| H                               | 1.35307  | 2.21026  | -1.35887 | H                             | -1.49703 | -1.71137 | 0.87457  |
| H                               | -1.85684 | 2.22106  | -0.44188 | H                             | 1.49703  | 1.71137  | 0.87457  |
| H                               | 0.55421  | 2.18984  | 1.83553  |                               |          |          |          |
| H                               | -1.35307 | -2.21026 | -1.35887 |                               |          |          |          |
| H                               | 1.85684  | -2.22106 | -0.44188 |                               |          |          |          |
| H                               | -0.55421 | -2.18984 | 1.83553  |                               |          |          |          |
| CH <sub>3</sub> NH <sub>2</sub> |          |          |          | N <sub>2</sub> H <sub>4</sub> |          |          |          |
| C                               | 1.33951  | -0.00070 | 0.03120  | N                             | 0.00000  | 1.37708  | -0.20748 |
| H                               | 2.04372  | -0.92907 | 1.74153  | N                             | 0.00000  | -1.37708 | -0.20748 |
| H                               | 2.19294  | -0.96582 | -1.58022 | H                             | -0.96419 | 2.03046  | 1.32720  |
| H                               | 2.03724  | 1.93417  | 0.01895  | H                             | 1.80702  | 1.91729  | 0.12516  |
| N                               | -1.41358 | -0.00210 | -0.21485 | H                             | -1.80702 | -1.91729 | 0.12516  |
| H                               | -2.21316 | -1.55623 | 0.54764  | H                             | 0.96419  | -2.03046 | 1.32720  |
| H                               | -2.20273 | 1.53584  | 0.58885  |                               |          |          |          |
| CH <sub>3</sub> OH              |          |          |          | NH <sub>2</sub> OH            |          |          |          |
| C                               | 1.26105  | 0.03603  | 0.00360  | N                             | 1.32103  | 0.11075  | -0.26947 |
| H                               | 2.05037  | -1.59094 | -0.97676 | O                             | -1.37881 | -0.23046 | 0.10707  |
| H                               | 2.01397  | 0.09183  | 1.92642  | H                             | -2.08376 | 1.35490  | -0.43181 |
| H                               | 1.86966  | 1.73491  | -0.99747 | H                             | 1.99895  | -1.58788 | 0.31497  |
| O                               | -1.41493 | -0.23255 | 0.00290  | H                             | 1.86810  | 1.30143  | 1.14659  |
| H                               | -2.18085 | 1.40841  | 0.00303  |                               |          |          |          |

Table S3: Geometries used for the B3P86 calculations.

| C <sub>2</sub> H <sub>6</sub>   |          |          |          | H <sub>2</sub> O <sub>2</sub> |          |          |          |
|---------------------------------|----------|----------|----------|-------------------------------|----------|----------|----------|
| C                               | 0.00000  | 1.44102  | -0.00579 | O                             | 0.00000  | 1.35232  | -0.11111 |
| C                               | 0.00000  | -1.44102 | -0.00579 | O                             | 0.00000  | -1.35232 | -0.11111 |
| H                               | 1.35296  | 2.20217  | -1.35876 | H                             | -1.48085 | -1.70194 | 0.88888  |
| H                               | -1.85665 | 2.21315  | -0.44194 | H                             | 1.48085  | 1.70194  | 0.88888  |
| H                               | 0.55408  | 2.18168  | 1.83542  |                               |          |          |          |
| H                               | -1.35296 | -2.20217 | -1.35876 |                               |          |          |          |
| H                               | 1.85665  | -2.21315 | -0.44194 |                               |          |          |          |
| H                               | -0.55408 | -2.18168 | 1.83542  |                               |          |          |          |
| CH <sub>3</sub> NH <sub>2</sub> |          |          |          | N <sub>2</sub> H <sub>4</sub> |          |          |          |
| C                               | 1.33132  | -0.00087 | 0.03135  | N                             | 0.00000  | 1.36577  | -0.20758 |
| H                               | 2.03676  | -0.93482 | 1.73811  | N                             | 0.00000  | -1.36577 | -0.20758 |
| H                               | 2.19038  | -0.95833 | -1.58192 | H                             | -0.95857 | 2.02123  | 1.32828  |
| H                               | 2.03175  | 1.93297  | 0.02714  | H                             | 1.80528  | 1.90709  | 0.12475  |
| N                               | -1.40746 | -0.00206 | -0.21651 | H                             | -1.80528 | -1.90709 | 0.12475  |
| H                               | -2.20316 | -1.55365 | 0.55103  | H                             | 0.95857  | -2.02123 | 1.32828  |
| H                               | -2.19143 | 1.53347  | 0.59311  |                               |          |          |          |
| CH <sub>3</sub> OH              |          |          |          | NH <sub>2</sub> OH            |          |          |          |
| C                               | 1.25082  | 0.03566  | 0.00386  | N                             | 1.30557  | 0.11121  | -0.27002 |
| H                               | 2.04817  | -1.58872 | -0.97565 | O                             | -1.36511 | -0.23058 | 0.10786  |
| H                               | 2.01059  | 0.09423  | 1.92499  | H                             | -2.07163 | 1.35044  | -0.43038 |
| H                               | 1.86381  | 1.73309  | -0.99885 | H                             | 1.99236  | -1.58299 | 0.31326  |
| O                               | -1.40744 | -0.23247 | 0.00291  | H                             | 1.86112  | 1.29869  | 1.14442  |
| H                               | -2.16792 | 1.40720  | 0.00303  |                               |          |          |          |

Table S4: Geometries used for the B3PW91 calculations.

| C <sub>2</sub> H <sub>6</sub>   |          |          |          | H <sub>2</sub> O <sub>2</sub> |          |          |          |
|---------------------------------|----------|----------|----------|-------------------------------|----------|----------|----------|
| C                               | 0.00000  | 1.44325  | -0.00579 | O                             | 0.00000  | 1.35394  | -0.11115 |
| C                               | 0.00000  | -1.44325 | -0.00579 | O                             | 0.00000  | -1.35394 | -0.11115 |
| H                               | 1.35411  | 2.20562  | -1.35991 | H                             | -1.48109 | -1.70354 | 0.88920  |
| H                               | -1.85821 | 2.21665  | -0.44227 | H                             | 1.48109  | 1.70354  | 0.88920  |
| H                               | 0.55461  | 2.18517  | 1.83694  |                               |          |          |          |
| H                               | -1.35411 | -2.20562 | -1.35991 |                               |          |          |          |
| H                               | 1.85821  | -2.21665 | -0.44227 |                               |          |          |          |
| H                               | -0.55461 | -2.18517 | 1.83694  |                               |          |          |          |
| CH <sub>3</sub> NH <sub>2</sub> |          |          |          | N <sub>2</sub> H <sub>4</sub> |          |          |          |
| C                               | 1.33281  | -0.00082 | 0.03132  | N                             | 0.00000  | 1.36715  | -0.20777 |
| H                               | 2.03972  | -0.93551 | 1.73957  | N                             | 0.00000  | -1.36715 | -0.20777 |
| H                               | 2.19322  | -0.95946 | -1.58312 | H                             | -0.95833 | 2.02274  | 1.32962  |
| H                               | 2.03495  | 1.93445  | 0.02690  | H                             | 1.80641  | 1.90824  | 0.12476  |
| N                               | -1.40928 | -0.00204 | -0.21654 | H                             | -1.80641 | -1.90824 | 0.12476  |
| H                               | -2.20565 | -1.55429 | 0.55116  | H                             | 0.95833  | -2.02274 | 1.32962  |
| H                               | -2.19415 | 1.53399  | 0.59330  |                               |          |          |          |
| CH <sub>3</sub> OH              |          |          |          | NH <sub>2</sub> OH            |          |          |          |
| C                               | 1.25177  | 0.03560  | 0.00385  | N                             | 1.30699  | 0.11122  | -0.27019 |
| H                               | 2.04848  | -1.59082 | -0.97708 | O                             | -1.36665 | -0.23058 | 0.10789  |
| H                               | 2.01269  | 0.09274  | 1.92680  | H                             | -2.07249 | 1.35132  | -0.43063 |
| H                               | 1.86713  | 1.73439  | -0.99925 | H                             | 1.99352  | -1.58426 | 0.31347  |
| O                               | -1.40905 | -0.23240 | 0.00290  | H                             | 1.86322  | 1.29903  | 1.14540  |
| H                               | -2.16657 | 1.40929  | 0.00327  |                               |          |          |          |

Table S5: Geometries used for the B97D calculations.

| C <sub>2</sub> H <sub>6</sub>   |          |          |          | H <sub>2</sub> O <sub>2</sub> |          |          |          |
|---------------------------------|----------|----------|----------|-------------------------------|----------|----------|----------|
| C                               | 0.00000  | 1.45587  | -0.00572 | O                             | 0.00000  | 1.38280  | -0.11385 |
| C                               | 0.00000  | -1.45587 | -0.00572 | O                             | 0.00000  | -1.38280 | -0.11385 |
| H                               | 1.36305  | 2.21562  | -1.36879 | H                             | -1.48494 | -1.70561 | 0.91079  |
| H                               | -1.87063 | 2.22585  | -0.44654 | H                             | 1.48494  | 1.70561  | 0.91079  |
| H                               | 0.55647  | 2.19477  | 1.84965  |                               |          |          |          |
| H                               | -1.36305 | -2.21562 | -1.36879 |                               |          |          |          |
| H                               | 1.87063  | -2.22585 | -0.44654 |                               |          |          |          |
| H                               | -0.55647 | -2.19477 | 1.84965  |                               |          |          |          |
| CH <sub>3</sub> NH <sub>2</sub> |          |          |          | N <sub>2</sub> H <sub>4</sub> |          |          |          |
| C                               | 1.34639  | -0.00011 | 0.03150  | N                             | 0.00000  | 1.38704  | -0.21195 |
| H                               | 2.04637  | -0.96907 | 1.73700  | N                             | 0.00000  | -1.38704 | -0.21195 |
| H                               | 2.20564  | -0.94168 | -1.60687 | H                             | -0.93617 | 2.02687  | 1.35995  |
| H                               | 2.03723  | 1.94965  | 0.05915  | H                             | 1.82348  | 1.90450  | 0.12372  |
| N                               | -1.42516 | -0.00240 | -0.22546 | H                             | -1.82348 | -1.90450 | 0.12372  |
| H                               | -2.20154 | -1.55684 | 0.57932  | H                             | 0.93617  | -2.02687 | 1.35995  |
| H                               | -2.18988 | 1.53537  | 0.62066  |                               |          |          |          |
| CH <sub>3</sub> OH              |          |          |          | NH <sub>2</sub> OH            |          |          |          |
| C                               | 1.26793  | 0.03433  | 0.00335  | N                             | -1.32897 | -0.11662 | -0.28572 |
| H                               | 2.05738  | -1.60733 | -0.98108 | O                             | 1.39410  | 0.23876  | 0.11744  |
| H                               | 2.02618  | 0.09714  | 1.94043  | H                             | 2.08212  | -1.35606 | -0.43921 |
| H                               | 1.87701  | 1.74357  | -1.00963 | H                             | -2.00213 | 1.58991  | 0.31605  |
| O                               | -1.42590 | -0.23354 | 0.00368  | H                             | -1.86951 | -1.30086 | 1.15449  |
| H                               | -2.16095 | 1.42891  | 0.00078  |                               |          |          |          |

Table S6: Geometries used for the B97D3 calculations.

| C <sub>2</sub> H <sub>6</sub>   |          |          |          | H <sub>2</sub> O <sub>2</sub> |          |          |          |
|---------------------------------|----------|----------|----------|-------------------------------|----------|----------|----------|
| C                               | 0.00000  | 1.45104  | -0.00586 | O                             | 0.00000  | 1.38276  | -0.11181 |
| C                               | 0.00000  | -1.45104 | -0.00586 | O                             | 0.00000  | -1.38276 | -0.11181 |
| H                               | 1.35925  | 2.21419  | -1.36512 | H                             | -1.49772 | -1.70445 | 0.89448  |
| H                               | -1.86529 | 2.22524  | -0.44367 | H                             | 1.49772  | 1.70445  | 0.89448  |
| H                               | 0.55690  | 2.19352  | 1.84396  |                               |          |          |          |
| H                               | -1.35925 | -2.21419 | -1.36512 |                               |          |          |          |
| H                               | 1.86529  | -2.22524 | -0.44367 |                               |          |          |          |
| H                               | -0.55690 | -2.19352 | 1.84396  |                               |          |          |          |
| CH <sub>3</sub> NH <sub>2</sub> |          |          |          | N <sub>2</sub> H <sub>4</sub> |          |          |          |
| C                               | 1.34310  | 0.00001  | 0.03193  | N                             | 0.00000  | 1.38514  | -0.21164 |
| H                               | 2.05021  | -0.96265 | 1.73427  | N                             | 0.00000  | -1.38514 | -0.21164 |
| H                               | 2.20080  | -0.94483 | -1.60146 | H                             | -0.93536 | 2.03149  | 1.35770  |
| H                               | 2.04027  | 1.94424  | 0.05071  | H                             | 1.82195  | 1.90572  | 0.12375  |
| N                               | -1.42162 | -0.00204 | -0.22357 | H                             | -1.82195 | -1.90572 | 0.12375  |
| H                               | -2.20450 | -1.55664 | 0.57295  | H                             | 0.93536  | -2.03149 | 1.35770  |
| H                               | -2.19401 | 1.53406  | 0.61698  |                               |          |          |          |
| CH <sub>3</sub> OH              |          |          |          | NH <sub>2</sub> OH            |          |          |          |
| C                               | 1.26577  | 0.03494  | 0.00354  | N                             | -1.32903 | -0.11790 | -0.28707 |
| H                               | 2.05468  | -1.60219 | -0.98068 | O                             | 1.39211  | 0.23795  | 0.11772  |
| H                               | 2.02531  | 0.09287  | 1.93569  | H                             | 2.08461  | -1.35474 | -0.44003 |
| H                               | 1.88026  | 1.73990  | -1.00503 | H                             | -2.00028 | 1.58799  | 0.31720  |
| O                               | -1.42353 | -0.23324 | 0.00332  | H                             | -1.87180 | -1.29818 | 1.15524  |
| H                               | -2.16665 | 1.42573  | 0.00218  |                               |          |          |          |

Table S7: Geometries used for the B98 calculations.

| C <sub>2</sub> H <sub>6</sub>   |          |          |          | H <sub>2</sub> O <sub>2</sub> |          |          |          |
|---------------------------------|----------|----------|----------|-------------------------------|----------|----------|----------|
| C                               | 0.00000  | 1.45032  | -0.00572 | O                             | 0.00000  | 1.35866  | -0.11059 |
| C                               | 0.00000  | -1.45032 | -0.00572 | O                             | 0.00000  | -1.35866 | -0.11059 |
| H                               | 1.35567  | 2.21050  | -1.36140 | H                             | -1.48487 | -1.70498 | 0.88475  |
| H                               | -1.86028 | 2.22110  | -0.44383 | H                             | 1.48487  | 1.70498  | 0.88475  |
| H                               | 0.55394  | 2.19008  | 1.83955  |                               |          |          |          |
| H                               | -1.35567 | -2.21050 | -1.36140 |                               |          |          |          |
| H                               | 1.86028  | -2.22110 | -0.44383 |                               |          |          |          |
| H                               | -0.55394 | -2.19008 | 1.83955  |                               |          |          |          |
| CH <sub>3</sub> NH <sub>2</sub> |          |          |          | N <sub>2</sub> H <sub>4</sub> |          |          |          |
| C                               | 1.33959  | -0.00057 | 0.03157  | N                             | 0.00000  | 1.37757  | -0.20880 |
| H                               | 2.04123  | -0.94415 | 1.73740  | N                             | 0.00000  | -1.37757 | -0.20880 |
| H                               | 2.19352  | -0.95529 | -1.58900 | H                             | -0.95325 | 2.02524  | 1.33704  |
| H                               | 2.03647  | 1.93736  | 0.03414  | H                             | 1.81088  | 1.91030  | 0.12455  |
| N                               | -1.41526 | -0.00195 | -0.21874 | H                             | -1.81088 | -1.91030 | 0.12455  |
| H                               | -2.20639 | -1.55483 | 0.55841  | H                             | 0.95325  | -2.02524 | 1.33704  |
| H                               | -2.19558 | 1.53398  | 0.60082  |                               |          |          |          |
| CH <sub>3</sub> OH              |          |          |          | NH <sub>2</sub> OH            |          |          |          |
| C                               | 1.25521  | 0.03570  | 0.00372  | N                             | 1.31564  | 0.11158  | -0.27062 |
| H                               | 2.04903  | -1.59273 | -0.97791 | O                             | -1.37420 | -0.23033 | 0.10739  |
| H                               | 2.01327  | 0.09220  | 1.92859  | H                             | -2.07556 | 1.35305  | -0.43192 |
| H                               | 1.86865  | 1.73631  | -0.99934 | H                             | 1.99533  | -1.58772 | 0.31488  |
| O                               | -1.41134 | -0.23230 | 0.00290  | H                             | 1.86430  | 1.29625  | 1.15226  |
| H                               | -2.17147 | 1.40841  | 0.00313  |                               |          |          |          |

Table S8: Geometries used for the B972 calculations.

| C <sub>2</sub> H <sub>6</sub>   |          |          |          | H <sub>2</sub> O <sub>2</sub> |          |          |          |
|---------------------------------|----------|----------|----------|-------------------------------|----------|----------|----------|
| C                               | 0.00000  | 1.44264  | -0.00569 | O                             | 0.00000  | 1.34899  | -0.11125 |
| C                               | 0.00000  | -1.44264 | -0.00569 | O                             | 0.00000  | -1.34899 | -0.11125 |
| H                               | 1.35254  | 2.20337  | -1.35823 | H                             | -1.47195 | -1.70034 | 0.88999  |
| H                               | -1.85572 | 2.21482  | -0.44206 | H                             | 1.47195  | 1.70034  | 0.88999  |
| H                               | 0.55426  | 2.18358  | 1.83443  |                               |          |          |          |
| H                               | -1.35254 | -2.20337 | -1.35823 |                               |          |          |          |
| H                               | 1.85572  | -2.21482 | -0.44206 |                               |          |          |          |
| H                               | -0.55426 | -2.18358 | 1.83443  |                               |          |          |          |
| CH <sub>3</sub> NH <sub>2</sub> |          |          |          | N <sub>2</sub> H <sub>4</sub> |          |          |          |
| C                               | 1.33105  | -0.00062 | 0.03135  | N                             | 0.00000  | 1.36470  | -0.20747 |
| H                               | 2.03677  | -0.94027 | 1.73343  | N                             | 0.00000  | -1.36470 | -0.20747 |
| H                               | 2.18880  | -0.95341 | -1.58370 | H                             | -0.95285 | 2.01789  | 1.32805  |
| H                               | 2.03156  | 1.93187  | 0.03278  | H                             | 1.80186  | 1.90298  | 0.12423  |
| N                               | -1.40834 | -0.00195 | -0.21750 | H                             | -1.80186 | -1.90298 | 0.12423  |
| H                               | -2.19815 | -1.54889 | 0.55459  | H                             | 0.95285  | -2.01789 | 1.32805  |
| H                               | -2.18688 | 1.52810  | 0.59734  |                               |          |          |          |
| CH <sub>3</sub> OH              |          |          |          | NH <sub>2</sub> OH            |          |          |          |
| C                               | 1.25050  | 0.03517  | 0.00380  | N                             | 1.30381  | 0.11121  | -0.26981 |
| H                               | 2.04615  | -1.58894 | -0.97470 | O                             | -1.36333 | -0.22968 | 0.10761  |
| H                               | 2.00968  | 0.09371  | 1.92376  | H                             | -2.06775 | 1.34536  | -0.42918 |
| H                               | 1.86450  | 1.73115  | -0.99822 | H                             | 1.98909  | -1.57890 | 0.31274  |
| O                               | -1.40782 | -0.23151 | 0.00296  | H                             | 1.85865  | 1.29256  | 1.14420  |
| H                               | -2.16078 | 1.40510  | 0.00266  |                               |          |          |          |

Table S9: Geometries used for the BLYP calculations.

| C <sub>2</sub> H <sub>6</sub>   |          |          |          | H <sub>2</sub> O <sub>2</sub> |          |          |          |
|---------------------------------|----------|----------|----------|-------------------------------|----------|----------|----------|
| C                               | 0.00000  | 1.45846  | -0.00574 | O                             | 0.00000  | 1.40619  | -0.10945 |
| C                               | 0.00000  | -1.45846 | -0.00574 | O                             | 0.00000  | -1.40619 | -0.10945 |
| H                               | 1.36149  | 2.22399  | -1.36724 | H                             | -1.52917 | -1.71660 | 0.87557  |
| H                               | -1.86814 | 2.23476  | -0.44566 | H                             | 1.52917  | 1.71660  | 0.87557  |
| H                               | 0.55649  | 2.20375  | 1.84737  |                               |          |          |          |
| H                               | -1.36149 | -2.22399 | -1.36724 |                               |          |          |          |
| H                               | 1.86814  | -2.23476 | -0.44566 |                               |          |          |          |
| H                               | -0.55649 | -2.20375 | 1.84737  |                               |          |          |          |
| CH <sub>3</sub> NH <sub>2</sub> |          |          |          | N <sub>2</sub> H <sub>4</sub> |          |          |          |
| C                               | 1.35384  | -0.00027 | 0.03210  | N                             | 0.00000  | 1.40162  | -0.21223 |
| H                               | 2.06082  | -0.95779 | 1.73996  | N                             | 0.00000  | -1.40162 | -0.21223 |
| H                               | 2.20823  | -0.95161 | -1.60228 | H                             | -0.94502 | 2.04700  | 1.36082  |
| H                               | 2.04931  | 1.94750  | 0.04344  | H                             | 1.83102  | 1.91960  | 0.12483  |
| N                               | -1.42987 | -0.00210 | -0.22271 | H                             | -1.83102 | -1.91960 | 0.12483  |
| H                               | -2.22166 | -1.56407 | 0.57108  | H                             | 0.94502  | -2.04700 | 1.36082  |
| H                               | -2.21069 | 1.54229  | 0.61413  |                               |          |          |          |
| CH <sub>3</sub> OH              |          |          |          | NH <sub>2</sub> OH            |          |          |          |
| C                               | 1.27928  | 0.03586  | 0.00352  | N                             | -1.34898 | -0.11829 | -0.29027 |
| H                               | 2.06023  | -1.60548 | -0.98435 | O                             | 1.41304  | 0.24232  | 0.11813  |
| H                               | 2.03351  | 0.08884  | 1.93939  | H                             | 2.10506  | -1.36383 | -0.44428 |
| H                               | 1.89045  | 1.74400  | -1.00470 | H                             | -2.01083 | 1.59896  | 0.31860  |
| O                               | -1.43408 | -0.23451 | 0.00316  | H                             | -1.88267 | -1.30404 | 1.16087  |
| H                               | -2.18724 | 1.43360  | 0.00329  |                               |          |          |          |

Table S10: Geometries used for the CAM-B3LYP calculations.

| C <sub>2</sub> H <sub>6</sub>   |          |          |          | H <sub>2</sub> O <sub>2</sub> |          |          |          |
|---------------------------------|----------|----------|----------|-------------------------------|----------|----------|----------|
| C                               | 0.00000  | 1.44226  | -0.00574 | O                             | 0.00000  | 1.35056  | -0.10911 |
| C                               | 0.00000  | -1.44226 | -0.00574 | O                             | 0.00000  | -1.35056 | -0.10911 |
| H                               | 1.35188  | 2.20177  | -1.35763 | H                             | -1.48989 | -1.71056 | 0.87285  |
| H                               | -1.85527 | 2.21238  | -0.44200 | H                             | 1.48989  | 1.71056  | 0.87285  |
| H                               | 0.55312  | 2.18138  | 1.83405  |                               |          |          |          |
| H                               | -1.35188 | -2.20177 | -1.35763 |                               |          |          |          |
| H                               | 1.85527  | -2.21238 | -0.44200 |                               |          |          |          |
| H                               | -0.55312 | -2.18138 | 1.83405  |                               |          |          |          |
| CH <sub>3</sub> NH <sub>2</sub> |          |          |          | N <sub>2</sub> H <sub>4</sub> |          |          |          |
| C                               | 1.33491  | -0.00113 | 0.03086  | N                             | 0.00000  | 1.36600  | -0.20512 |
| H                               | 2.03350  | -0.91348 | 1.74783  | N                             | 0.00000  | -1.36600 | -0.20512 |
| H                               | 2.18703  | -0.97715 | -1.57062 | H                             | -0.98216 | 2.02444  | 1.30974  |
| H                               | 2.03233  | 1.93121  | 0.00329  | H                             | 1.79920  | 1.92060  | 0.12609  |
| N                               | -1.40666 | -0.00196 | -0.21051 | H                             | -1.79920 | -1.92060 | 0.12609  |
| H                               | -2.21279 | -1.55736 | 0.53328  | H                             | 0.98216  | -2.02444 | 1.30974  |
| H                               | -2.20295 | 1.53731  | 0.57462  |                               |          |          |          |
| CH <sub>3</sub> OH              |          |          |          | NH <sub>2</sub> OH            |          |          |          |
| C                               | 1.25392  | 0.03657  | 0.00376  | N                             | -1.30805 | -0.10623 | -0.26068 |
| H                               | 2.04733  | -1.58580 | -0.97646 | O                             | 1.36373  | 0.22902  | 0.09972  |
| H                               | 2.00636  | 0.09135  | 1.92397  | H                             | 2.07923  | -1.35130 | -0.42778 |
| H                               | 1.86062  | 1.73496  | -0.99489 | H                             | -1.99703 | 1.58800  | 0.31171  |
| O                               | -1.40682 | -0.23246 | 0.00258  | H                             | -1.86227 | -1.30435 | 1.14009  |
| H                               | -2.18328 | 1.39976  | 0.00418  |                               |          |          |          |

Table S11: Geometries used for the HF calculations.

| C <sub>2</sub> H <sub>6</sub>   |          |          |          | H <sub>2</sub> O <sub>2</sub> |          |          |          |
|---------------------------------|----------|----------|----------|-------------------------------|----------|----------|----------|
| C                               | 0.00000  | 1.44540  | -0.00580 | O                             | 0.00000  | 1.30749  | -0.10823 |
| C                               | 0.00000  | -1.44540 | -0.00580 | O                             | 0.00000  | -1.30749 | -0.10823 |
| H                               | 1.34610  | 2.19640  | -1.35180 | H                             | -1.43216 | -1.71197 | 0.86584  |
| H                               | -1.84760 | 2.20620  | -0.44010 | H                             | 1.43216  | 1.71197  | 0.86584  |
| H                               | 0.55040  | 2.17530  | 1.82660  |                               |          |          |          |
| H                               | -1.34610 | -2.19640 | -1.35180 |                               |          |          |          |
| H                               | 1.84760  | -2.20620 | -0.44010 |                               |          |          |          |
| H                               | -0.55040 | -2.17530 | 1.82660  |                               |          |          |          |
| CH <sub>3</sub> NH <sub>2</sub> |          |          |          | N <sub>2</sub> H <sub>4</sub> |          |          |          |
| C                               | 1.33101  | -0.00054 | 0.02964  | N                             | 0.00000  | 1.35037  | -0.20021 |
| H                               | 2.01489  | -0.90873 | 1.73946  | N                             | 0.00000  | -1.35037 | -0.20021 |
| H                               | 2.17263  | -0.97895 | -1.55898 | H                             | -0.98949 | 2.00361  | 1.27599  |
| H                               | 2.02662  | 1.92027  | 0.00228  | H                             | 1.76927  | 1.91419  | 0.12549  |
| N                               | -1.40275 | -0.00171 | -0.20840 | H                             | -1.76927 | -1.91419 | 0.12549  |
| H                               | -2.19560 | -1.53762 | 0.53035  | H                             | 0.98949  | -2.00361 | 1.27599  |
| H                               | -2.18535 | 1.52020  | 0.56785  |                               |          |          |          |
| CH <sub>3</sub> OH              |          |          |          | NH <sub>2</sub> OH            |          |          |          |
| C                               | 1.24039  | 0.03557  | 0.00335  | N                             | 1.27399  | 0.10096  | -0.25903 |
| H                               | 2.03753  | -1.57435 | -0.96644 | O                             | -1.33395 | -0.22509 | 0.10739  |
| H                               | 1.98362  | 0.09647  | 1.91184  | H                             | -2.08200 | 1.29409  | -0.42079 |
| H                               | 1.83931  | 1.72624  | -0.98743 | H                             | 1.99556  | -1.54353 | 0.32078  |
| O                               | -1.39102 | -0.22772 | 0.00252  | H                             | 1.84015  | 1.34342  | 1.05410  |
| H                               | -2.17467 | 1.36000  | 0.00181  |                               |          |          |          |

Table S12: Geometries used for the LSDA calculations.

| C <sub>2</sub> H <sub>6</sub>   |          |          |          | H <sub>2</sub> O <sub>2</sub> |          |          |          |
|---------------------------------|----------|----------|----------|-------------------------------|----------|----------|----------|
| C                               | 0.00000  | 1.42835  | -0.00640 | O                             | 0.00000  | 1.34816  | -0.11290 |
| C                               | 0.00000  | -1.42835 | -0.00640 | O                             | 0.00000  | -1.34816 | -0.11290 |
| H                               | 1.36056  | 2.20534  | -1.36696 | H                             | -1.49701 | -1.70079 | 0.90323  |
| H                               | -1.86779 | 2.21773  | -0.43886 | H                             | 1.49701  | 1.70079  | 0.90323  |
| H                               | 0.56324  | 2.18323  | 1.84420  |                               |          |          |          |
| H                               | -1.36056 | -2.20534 | -1.36696 |                               |          |          |          |
| H                               | 1.86779  | -2.21773 | -0.43886 |                               |          |          |          |
| H                               | -0.56324 | -2.18323 | 1.84420  |                               |          |          |          |
| CH <sub>3</sub> NH <sub>2</sub> |          |          |          | N <sub>2</sub> H <sub>4</sub> |          |          |          |
| C                               | 1.31775  | -0.00152 | 0.03196  | N                             | 0.00000  | 1.35315  | -0.20794 |
| H                               | 2.05366  | -0.90483 | 1.76539  | N                             | 0.00000  | -1.35315 | -0.20794 |
| H                               | 2.19571  | -0.98979 | -1.57656 | H                             | -0.97637 | 2.03869  | 1.32907  |
| H                               | 2.03224  | 1.94426  | -0.01476 | H                             | 1.81659  | 1.91815  | 0.12647  |
| N                               | -1.39344 | -0.00246 | -0.20778 | H                             | -1.81659 | -1.91815 | 0.12647  |
| H                               | -2.22236 | -1.57486 | 0.52034  | H                             | 0.97637  | -2.03869 | 1.32907  |
| H                               | -2.21168 | 1.55159  | 0.56829  |                               |          |          |          |
| CH <sub>3</sub> OH              |          |          |          | NH <sub>2</sub> OH            |          |          |          |
| C                               | 1.23804  | 0.03720  | 0.00452  | N                             | 1.29393  | 0.11331  | -0.27365 |
| H                               | 2.05401  | -1.59602 | -0.98463 | O                             | -1.35619 | -0.23400 | 0.11037  |
| H                               | 2.02178  | 0.09551  | 1.93742  | H                             | -2.07725 | 1.36067  | -0.43229 |
| H                               | 1.86895  | 1.74446  | -1.00833 | H                             | 2.00126  | -1.59160 | 0.31254  |
| O                               | -1.39925 | -0.23556 | 0.00294  | H                             | 1.86800  | 1.30975  | 1.15236  |
| H                               | -2.17902 | 1.41732  | 0.00493  |                               |          |          |          |

Table S13: Geometries used for the M06 calculations.

| C <sub>2</sub> H <sub>6</sub>   |          |          |          | H <sub>2</sub> O <sub>2</sub> |          |          |          |
|---------------------------------|----------|----------|----------|-------------------------------|----------|----------|----------|
| C                               | 0.00000  | 1.43781  | -0.00571 | O                             | 0.00000  | 1.34143  | -0.11126 |
| C                               | 0.00000  | -1.43781 | -0.00571 | O                             | 0.00000  | -1.34143 | -0.11126 |
| H                               | 1.35195  | 2.19709  | -1.35767 | H                             | -1.47486 | -1.70308 | 0.89006  |
| H                               | -1.85532 | 2.20757  | -0.44248 | H                             | 1.47486  | 1.70308  | 0.89006  |
| H                               | 0.55264  | 2.17650  | 1.83443  |                               |          |          |          |
| H                               | -1.35195 | -2.19709 | -1.35767 |                               |          |          |          |
| H                               | 1.85532  | -2.20757 | -0.44248 |                               |          |          |          |
| H                               | -0.55264 | -2.17650 | 1.83443  |                               |          |          |          |
| CH <sub>3</sub> NH <sub>2</sub> |          |          |          | N <sub>2</sub> H <sub>4</sub> |          |          |          |
| C                               | 1.33025  | -0.00106 | 0.03115  | N                             | 0.00000  | 1.36448  | -0.20717 |
| H                               | 2.03470  | -0.92237 | 1.74235  | N                             | 0.00000  | -1.36448 | -0.20717 |
| H                               | 2.18909  | -0.96673 | -1.57506 | H                             | -0.96080 | 2.01814  | 1.32552  |
| H                               | 2.02761  | 1.93167  | 0.01481  | H                             | 1.80254  | 1.90812  | 0.12465  |
| N                               | -1.40451 | -0.00232 | -0.21319 | H                             | -1.80254 | -1.90812 | 0.12465  |
| H                               | -2.20649 | -1.55394 | 0.54104  | H                             | 0.96080  | -2.01814 | 1.32552  |
| H                               | -2.19481 | 1.53399  | 0.58233  |                               |          |          |          |
| CH <sub>3</sub> OH              |          |          |          | NH <sub>2</sub> OH            |          |          |          |
| C                               | 1.24433  | 0.03605  | 0.00379  | N                             | 1.29791  | 0.11100  | -0.26996 |
| H                               | 2.04676  | -1.58476 | -0.97513 | O                             | -1.35795 | -0.23055 | 0.10845  |
| H                               | 2.00838  | 0.09331  | 1.92181  | H                             | -2.07515 | 1.34296  | -0.42915 |
| H                               | 1.85939  | 1.73227  | -0.99601 | H                             | 1.99446  | -1.57733 | 0.31366  |
| O                               | -1.40148 | -0.23223 | 0.00287  | H                             | 1.85888  | 1.30170  | 1.13765  |
| H                               | -2.16866 | 1.40068  | 0.00371  |                               |          |          |          |

Table S14: Geometries used for the M06-2X calculations.

| C <sub>2</sub> H <sub>6</sub>   |          |          |          | H <sub>2</sub> O <sub>2</sub> |          |          |          |
|---------------------------------|----------|----------|----------|-------------------------------|----------|----------|----------|
| C                               | 0.00000  | 1.44375  | -0.00586 | O                             | 0.00000  | 1.35960  | -0.08977 |
| C                               | 0.00000  | -1.44375 | -0.00586 | O                             | 0.00000  | -1.35960 | -0.08977 |
| H                               | 1.35165  | 2.20135  | -1.35752 | H                             | -1.55209 | -1.83725 | 0.71819  |
| H                               | -1.85504 | 2.21233  | -0.44094 | H                             | 1.55209  | 1.83725  | 0.71819  |
| H                               | 0.55404  | 2.18022  | 1.83362  |                               |          |          |          |
| H                               | -1.35165 | -2.20135 | -1.35752 |                               |          |          |          |
| H                               | 1.85504  | -2.21233 | -0.44094 |                               |          |          |          |
| H                               | -0.55404 | -2.18022 | 1.83362  |                               |          |          |          |
| CH <sub>3</sub> NH <sub>2</sub> |          |          |          | N <sub>2</sub> H <sub>4</sub> |          |          |          |
| C                               | 1.33601  | -0.00098 | 0.03149  | N                             | 0.00000  | 1.36701  | -0.20727 |
| H                               | 2.03111  | -0.93644 | 1.73525  | N                             | 0.00000  | -1.36701 | -0.20727 |
| H                               | 2.18654  | -0.95635 | -1.58170 | H                             | -0.96000 | 2.01677  | 1.32608  |
| H                               | 2.03093  | 1.93142  | 0.02949  | H                             | 1.80413  | 1.90863  | 0.12484  |
| N                               | -1.41009 | -0.00180 | -0.21709 | H                             | -1.80413 | -1.90863 | 0.12484  |
| H                               | -2.20230 | -1.55313 | 0.55297  | H                             | 0.96000  | -2.01677 | 1.32608  |
| H                               | -2.19172 | 1.53298  | 0.59468  |                               |          |          |          |
| CH <sub>3</sub> OH              |          |          |          | NH <sub>2</sub> OH            |          |          |          |
| C                               | 1.25238  | 0.03602  | 0.00390  | N                             | 1.30003  | 0.11047  | -0.26897 |
| H                               | 2.04624  | -1.58666 | -0.97388 | O                             | -1.35914 | -0.23063 | 0.10809  |
| H                               | 2.00358  | 0.09486  | 1.92311  | H                             | -2.07930 | 1.34246  | -0.42909 |
| H                               | 1.85921  | 1.73206  | -0.99694 | H                             | 1.99543  | -1.57836 | 0.31493  |
| O                               | -1.40624 | -0.23239 | 0.00274  | H                             | 1.85676  | 1.30765  | 1.13221  |
| H                               | -2.17342 | 1.40270  | 0.00240  |                               |          |          |          |

Table S15: Geometries used for the MN12-SX calculations.

| C <sub>2</sub> H <sub>6</sub>   |          |          |          | H <sub>2</sub> O <sub>2</sub> |          |          |          |
|---------------------------------|----------|----------|----------|-------------------------------|----------|----------|----------|
| C                               | 0.00000  | 1.43830  | -0.00589 | O                             | 0.00000  | 1.34823  | -0.11082 |
| C                               | 0.00000  | -1.43830 | -0.00589 | O                             | 0.00000  | -1.34823 | -0.11082 |
| H                               | 1.35180  | 2.19920  | -1.35770 | H                             | -1.47840 | -1.70162 | 0.88658  |
| H                               | -1.85520 | 2.21039  | -0.44066 | H                             | 1.47840  | 1.70162  | 0.88658  |
| H                               | 0.55455  | 2.17814  | 1.83371  |                               |          |          |          |
| H                               | -1.35180 | -2.19920 | -1.35770 |                               |          |          |          |
| H                               | 1.85520  | -2.21039 | -0.44066 |                               |          |          |          |
| H                               | -0.55455 | -2.17814 | 1.83371  |                               |          |          |          |
| CH <sub>3</sub> NH <sub>2</sub> |          |          |          | N <sub>2</sub> H <sub>4</sub> |          |          |          |
| C                               | 1.32642  | -0.00027 | 0.03190  | N                             | 0.00000  | 1.36648  | -0.20906 |
| H                               | 2.03577  | -0.94202 | 1.73151  | N                             | 0.00000  | -1.36648 | -0.20906 |
| H                               | 2.18722  | -0.95260 | -1.58310 | H                             | -0.94904 | 2.01893  | 1.33901  |
| H                               | 2.03001  | 1.93155  | 0.03516  | H                             | 1.81135  | 1.90136  | 0.12439  |
| N                               | -1.40410 | -0.00210 | -0.21948 | H                             | -1.81135 | -1.90136 | 0.12439  |
| H                               | -2.19675 | -1.55361 | 0.55997  | H                             | 0.94904  | -2.01893 | 1.33901  |
| H                               | -2.18606 | 1.53297  | 0.60141  |                               |          |          |          |
| CH <sub>3</sub> OH              |          |          |          | NH <sub>2</sub> OH            |          |          |          |
| C                               | 1.24027  | 0.03612  | 0.00392  | N                             | 1.30297  | 0.11197  | -0.27161 |
| H                               | 2.04396  | -1.58789 | -0.97208 | O                             | -1.36146 | -0.23029 | 0.10832  |
| H                               | 2.00751  | 0.10068  | 1.92219  | H                             | -2.07752 | 1.34398  | -0.42989 |
| H                               | 1.85920  | 1.72985  | -1.00142 | H                             | 1.98936  | -1.58539 | 0.31666  |
| O                               | -1.39759 | -0.23240 | 0.00341  | H                             | 1.85899  | 1.29991  | 1.14798  |
| H                               | -2.17155 | 1.39986  | 0.00053  |                               |          |          |          |

Table S16: Geometries used for the PBEP86 calculations.

| C <sub>2</sub> H <sub>6</sub>   |          |          |          | H <sub>2</sub> O <sub>2</sub> |          |          |          |
|---------------------------------|----------|----------|----------|-------------------------------|----------|----------|----------|
| C                               | 0.00000  | 1.45075  | -0.00595 | O                             | 0.00000  | 1.38572  | -0.11263 |
| C                               | 0.00000  | -1.45075 | -0.00595 | O                             | 0.00000  | -1.38572 | -0.11263 |
| H                               | 1.36454  | 2.22030  | -1.37050 | H                             | -1.50894 | -1.70758 | 0.90104  |
| H                               | -1.87259 | 2.23170  | -0.44469 | H                             | 1.50894  | 1.70758  | 0.90104  |
| H                               | 0.55991  | 2.19936  | 1.85092  |                               |          |          |          |
| H                               | -1.36454 | -2.22030 | -1.37050 |                               |          |          |          |
| H                               | 1.87259  | -2.23170 | -0.44469 |                               |          |          |          |
| H                               | -0.55991 | -2.19936 | 1.85092  |                               |          |          |          |
| CH <sub>3</sub> NH <sub>2</sub> |          |          |          | N <sub>2</sub> H <sub>4</sub> |          |          |          |
| C                               | 1.34276  | -0.00053 | 0.03262  | N                             | 0.00000  | 1.38596  | -0.21286 |
| H                               | 2.05947  | -0.96431 | 1.74138  | N                             | 0.00000  | -1.38596 | -0.21286 |
| H                               | 2.20815  | -0.94687 | -1.60795 | H                             | -0.93931 | 2.04104  | 1.36543  |
| H                               | 2.04545  | 1.95161  | 0.04915  | H                             | 1.83290  | 1.91106  | 0.12456  |
| N                               | -1.42177 | -0.00206 | -0.22422 | H                             | -1.83290 | -1.91106 | 0.12456  |
| H                               | -2.21446 | -1.56582 | 0.57269  | H                             | 0.93931  | -2.04104 | 1.36543  |
| H                               | -2.20272 | 1.54300  | 0.61852  |                               |          |          |          |
| CH <sub>3</sub> OH              |          |          |          | NH <sub>2</sub> OH            |          |          |          |
| C                               | 1.26538  | 0.03564  | 0.00389  | N                             | -1.32862 | -0.11850 | -0.29143 |
| H                               | 2.05970  | -1.60809 | -0.98584 | O                             | 1.39492  | 0.24206  | 0.11943  |
| H                               | 2.03340  | 0.09249  | 1.94319  | H                             | 2.09367  | -1.36141 | -0.44390 |
| H                               | 1.88708  | 1.74627  | -1.01009 | H                             | -2.00683 | 1.59667  | 0.31797  |
| O                               | -1.42486 | -0.23507 | 0.00331  | H                             | -1.87753 | -1.30369 | 1.16099  |
| H                               | -2.17354 | 1.43608  | 0.00296  |                               |          |          |          |

Table S17: Geometries used for the BHandHLYP calculations.

| C <sub>2</sub> H <sub>6</sub>   |          |          |          | H <sub>2</sub> O <sub>2</sub> |          |          |          |
|---------------------------------|----------|----------|----------|-------------------------------|----------|----------|----------|
| C                               | 0.00000  | 1.43913  | -0.00576 | O                             | 0.00000  | 1.33273  | -0.10853 |
| C                               | 0.00000  | -1.43913 | -0.00576 | O                             | 0.00000  | -1.33273 | -0.10853 |
| H                               | 1.34461  | 2.19320  | -1.35037 | H                             | -1.46407 | -1.70746 | 0.86823  |
| H                               | -1.84545 | 2.20356  | -0.43941 | H                             | 1.46407  | 1.70746  | 0.86823  |
| H                               | 0.55020  | 2.17250  | 1.82431  |                               |          |          |          |
| H                               | -1.34461 | -2.19320 | -1.35037 |                               |          |          |          |
| H                               | 1.84545  | -2.20356 | -0.43941 |                               |          |          |          |
| H                               | -0.55020 | -2.17250 | 1.82431  |                               |          |          |          |
| CH <sub>3</sub> NH <sub>2</sub> |          |          |          | N <sub>2</sub> H <sub>4</sub> |          |          |          |
| C                               | 1.32936  | -0.00093 | 0.03036  | N                             | 0.00000  | 1.35763  | -0.20273 |
| H                               | 2.02224  | -0.90881 | 1.73742  | N                             | 0.00000  | -1.35763 | -0.20273 |
| H                               | 2.17516  | -0.97306 | -1.56112 | H                             | -0.97962 | 2.01400  | 1.29369  |
| H                               | 2.02364  | 1.92001  | 0.00369  | H                             | 1.78280  | 1.91226  | 0.12545  |
| N                               | -1.40112 | -0.00196 | -0.20925 | H                             | -1.78280 | -1.91226 | 0.12545  |
| H                               | -2.19983 | -1.54468 | 0.53159  | H                             | 0.97962  | -2.01400 | 1.29369  |
| H                               | -2.18953 | 1.52582  | 0.57102  |                               |          |          |          |
| CH <sub>3</sub> OH              |          |          |          | NH <sub>2</sub> OH            |          |          |          |
| C                               | 1.24615  | 0.03606  | 0.00367  | N                             | 1.29127  | 0.10528  | -0.26341 |
| H                               | 2.03741  | -1.57590 | -0.96903 | O                             | -1.35065 | -0.22768 | 0.10739  |
| H                               | 1.99341  | 0.09288  | 1.91193  | H                             | -2.07976 | 1.32127  | -0.42565 |
| H                               | 1.84881  | 1.72437  | -0.98890 | H                             | 1.99527  | -1.56039 | 0.31713  |
| O                               | -1.39785 | -0.22990 | 0.00259  | H                             | 1.85077  | 1.32356  | 1.09325  |
| H                               | -2.17369 | 1.38154  | 0.00327  |                               |          |          |          |

Table S18: Geometries used for the LC-BLYP calculations.

| C <sub>2</sub> H <sub>6</sub>   |          |          |          | H <sub>2</sub> O <sub>2</sub> |          |          |          |
|---------------------------------|----------|----------|----------|-------------------------------|----------|----------|----------|
| C                               | 0.00000  | 1.43364  | -0.00585 | O                             | 0.00000  | 1.32722  | -0.10842 |
| C                               | 0.00000  | -1.43364 | -0.00585 | O                             | 0.00000  | -1.32722 | -0.10842 |
| H                               | 1.34996  | 2.19266  | -1.35582 | H                             | -1.48680 | -1.71561 | 0.86739  |
| H                               | -1.85307 | 2.20355  | -0.44007 | H                             | 1.48680  | 1.71561  | 0.86739  |
| H                               | 0.55359  | 2.17190  | 1.83100  |                               |          |          |          |
| H                               | -1.34996 | -2.19266 | -1.35582 |                               |          |          |          |
| H                               | 1.85307  | -2.20355 | -0.44007 |                               |          |          |          |
| H                               | -0.55359 | -2.17190 | 1.83100  |                               |          |          |          |
| CH <sub>3</sub> NH <sub>2</sub> |          |          |          | N <sub>2</sub> H <sub>4</sub> |          |          |          |
| C                               | 1.32650  | -0.00161 | 0.03002  | N                             | 0.00000  | 1.34983  | -0.20089 |
| H                               | 2.02659  | -0.86957 | 1.76666  | N                             | 0.00000  | -1.34983 | -0.20089 |
| H                               | 2.17929  | -1.01301 | -1.54636 | H                             | -1.01713 | 2.02350  | 1.27821  |
| H                               | 2.02854  | 1.92591  | -0.04519 | H                             | 1.78683  | 1.93474  | 0.12804  |
| N                               | -1.39410 | -0.00198 | -0.19875 | H                             | -1.78683 | -1.93474 | 0.12804  |
| H                               | -2.22140 | -1.56543 | 0.49725  | H                             | 1.01713  | -2.02350 | 1.27821  |
| H                               | -2.21330 | 1.54558  | 0.53879  |                               |          |          |          |
| CH <sub>3</sub> OH              |          |          |          | NH <sub>2</sub> OH            |          |          |          |
| C                               | 1.24601  | 0.03778  | 0.00396  | N                             | 1.28288  | 0.10462  | -0.26333 |
| H                               | 2.04609  | -1.57838 | -0.97697 | O                             | -1.34444 | -0.23102 | 0.10929  |
| H                               | 1.99703  | 0.09090  | 1.92188  | H                             | -2.09921 | 1.32729  | -0.42671 |
| H                               | 1.84747  | 1.73706  | -0.99151 | H                             | 2.01549  | -1.56483 | 0.31790  |
| O                               | -1.39644 | -0.23306 | 0.00209  | H                             | 1.85911  | 1.35333  | 1.07782  |
| H                               | -2.19513 | 1.38822  | 0.00618  |                               |          |          |          |

Table S19: Geometries used for the LC-B97D calculations.

| C <sub>2</sub> H <sub>6</sub>   |          |          |          | H <sub>2</sub> O <sub>2</sub> |          |          |          |
|---------------------------------|----------|----------|----------|-------------------------------|----------|----------|----------|
| C                               | 0.00000  | 1.44400  | -0.00578 | O                             | 0.00000  | 1.33843  | -0.10910 |
| C                               | 0.00000  | -1.44400 | -0.00578 | O                             | 0.00000  | -1.33843 | -0.10910 |
| H                               | 1.35512  | 2.19480  | -1.36092 | H                             | -1.48413 | -1.72196 | 0.87277  |
| H                               | -1.86056 | 2.20447  | -0.44298 | H                             | 1.48413  | 1.72196  | 0.87277  |
| H                               | 0.55399  | 2.17329  | 1.83861  |                               |          |          |          |
| H                               | -1.35512 | -2.19480 | -1.36092 |                               |          |          |          |
| H                               | 1.86056  | -2.20447 | -0.44298 |                               |          |          |          |
| H                               | -0.55399 | -2.17329 | 1.83861  |                               |          |          |          |
| CH <sub>3</sub> NH <sub>2</sub> |          |          |          | N <sub>2</sub> H <sub>4</sub> |          |          |          |
| C                               | 1.33775  | -0.00128 | 0.02949  | N                             | 0.00000  | 1.36008  | -0.20128 |
| H                               | 2.02281  | -0.87799 | 1.77101  | N                             | 0.00000  | -1.36008 | -0.20128 |
| H                               | 2.18390  | -1.01366 | -1.55284 | H                             | -1.01984 | 2.02236  | 1.28076  |
| H                               | 2.02663  | 1.93463  | -0.03758 | H                             | 1.78989  | 1.93631  | 0.12821  |
| N                               | -1.40361 | -0.00233 | -0.20097 | H                             | -1.78989 | -1.93631 | 0.12821  |
| H                               | -2.22184 | -1.56649 | 0.50519  | H                             | 1.01984  | -2.02236 | 1.28076  |
| H                               | -2.21270 | 1.54749  | 0.54404  |                               |          |          |          |
| CH <sub>3</sub> OH              |          |          |          | NH <sub>2</sub> OH            |          |          |          |
| C                               | 1.25698  | 0.03732  | 0.00352  | N                             | 1.29541  | 0.10350  | -0.26210 |
| H                               | 2.04995  | -1.58602 | -0.97716 | O                             | -1.35515 | -0.23048 | 0.10823  |
| H                               | 1.99831  | 0.09597  | 1.92817  | H                             | -2.10278 | 1.33094  | -0.42845 |
| H                               | 1.84572  | 1.74255  | -0.99645 | H                             | 2.01608  | -1.57043 | 0.32059  |
| O                               | -1.40425 | -0.23308 | 0.00255  | H                             | 1.86005  | 1.35887  | 1.07674  |
| H                               | -2.20186 | 1.38820  | 0.00395  |                               |          |          |          |

Table S20: Geometries used for the LC-BP86 calculations.

| C <sub>2</sub> H <sub>6</sub>   |          |          |          | H <sub>2</sub> O <sub>2</sub> |          |          |          |
|---------------------------------|----------|----------|----------|-------------------------------|----------|----------|----------|
| C                               | 0.00000  | 1.42861  | -0.00597 | O                             | 0.00000  | 1.31510  | -0.11054 |
| C                               | 0.00000  | -1.42861 | -0.00597 | O                             | 0.00000  | -1.31510 | -0.11054 |
| H                               | 1.35257  | 2.19045  | -1.35855 | H                             | -1.47294 | -1.70722 | 0.88430  |
| H                               | -1.85676 | 2.20177  | -0.43988 | H                             | 1.47294  | 1.70722  | 0.88430  |
| H                               | 0.55580  | 2.16928  | 1.83423  |                               |          |          |          |
| H                               | -1.35257 | -2.19045 | -1.35855 |                               |          |          |          |
| H                               | 1.85676  | -2.20177 | -0.43988 |                               |          |          |          |
| H                               | -0.55580 | -2.16928 | 1.83423  |                               |          |          |          |
| CH <sub>3</sub> NH <sub>2</sub> |          |          |          | N <sub>2</sub> H <sub>4</sub> |          |          |          |
| C                               | 1.31944  | -0.00187 | 0.03046  | N                             | 0.00000  | 1.34166  | -0.20214 |
| H                               | 2.02466  | -0.87995 | 1.76605  | N                             | 0.00000  | -1.34166 | -0.20214 |
| H                               | 2.18026  | -1.00474 | -1.55386 | H                             | -1.00696 | 2.01553  | 1.28756  |
| H                               | 2.02621  | 1.92948  | -0.03442 | H                             | 1.79020  | 1.92396  | 0.12741  |
| N                               | -1.38964 | -0.00192 | -0.20130 | H                             | -1.79020 | -1.92396 | 0.12741  |
| H                               | -2.21476 | -1.56573 | 0.50264  | H                             | 1.00696  | -2.01553 | 1.28756  |
| H                               | -2.20554 | 1.54560  | 0.54597  |                               |          |          |          |
| CH <sub>3</sub> OH              |          |          |          | NH <sub>2</sub> OH            |          |          |          |
| C                               | 1.23746  | 0.03754  | 0.00426  | N                             | 1.27119  | 0.10600  | -0.26516 |
| H                               | 2.04644  | -1.58005 | -0.97866 | O                             | -1.33422 | -0.23154 | 0.11017  |
| H                               | 1.99613  | 0.09277  | 1.92531  | H                             | -2.08587 | 1.32778  | -0.42645 |
| H                               | 1.84388  | 1.73942  | -0.99518 | H                             | 2.00793  | -1.56471 | 0.31621  |
| O                               | -1.39105 | -0.23359 | 0.00206  | H                             | 1.85333  | 1.34724  | 1.08505  |
| H                               | -2.18286 | 1.39138  | 0.00646  |                               |          |          |          |

## 2 Disaggregated data

Table S21: AD<sub>HV</sub>

| Functional | CH <sub>3</sub> -CH <sub>3</sub> | CH <sub>3</sub> -NH <sub>2</sub> | CH <sub>3</sub> -OH | NH <sub>2</sub> -NH <sub>2</sub> | NH <sub>2</sub> -OH | HO-OH     |
|------------|----------------------------------|----------------------------------|---------------------|----------------------------------|---------------------|-----------|
| APFD       | 5.033E-05                        | 1.953E-04                        | 1.863E-04           | 2.179E-04                        | 4.028E-04           | 3.039E-04 |
| B3LYP      | 5.291E-05                        | 2.082E-04                        | 1.982E-04           | 2.323E-04                        | 4.282E-04           | 3.656E-04 |
| B3P86      | 4.731E-05                        | 1.833E-04                        | 1.770E-04           | 2.031E-04                        | 3.784E-04           | 2.862E-04 |
| B3PW91     | 5.113E-05                        | 1.958E-04                        | 1.877E-04           | 2.156E-04                        | 4.025E-04           | 3.025E-04 |
| B97-2      | 5.101E-05                        | 1.970E-04                        | 1.881E-04           | 2.199E-04                        | 4.098E-04           | 3.070E-04 |
| B97D       | 6.037E-05                        | 2.271E-04                        | 2.218E-04           | 2.544E-04                        | 4.728E-04           | 4.012E-04 |
| B97D3      | 6.010E-05                        | 2.282E-04                        | 2.211E-04           | 2.551E-04                        | 4.728E-04           | 4.037E-04 |
| B98        | 5.121E-05                        | 1.954E-04                        | 1.877E-04           | 2.164E-04                        | 4.060E-04           | 3.049E-04 |
| BHandHLYP  | 4.438E-05                        | 1.782E-04                        | 2.849E-04           | 1.964E-04                        | 3.654E-04           | 2.681E-04 |
| BLYP       | 6.420E-05                        | 2.464E-04                        | 2.405E-04           | 2.729E-04                        | 4.993E-04           | 4.363E-04 |
| CAM-B3LYP  | 4.963E-05                        | 1.998E-04                        | 1.925E-04           | 2.235E-04                        | 4.227E-04           | 3.197E-04 |
| HF         | 3.855E-05                        | 1.540E-04                        | 1.404E-04           | 1.663E-04                        | 3.032E-04           | 2.184E-04 |
| LC-BLYP    | 4.496E-05                        | 1.868E-04                        | 1.819E-04           | 2.086E-04                        | 4.036E-04           | 3.068E-04 |
| LC-B97D    | 4.231E-05                        | 1.612E-04                        | 1.519E-04           | 1.701E-04                        | 3.260E-04           | 2.480E-04 |
| LC-BP86    | 4.204E-05                        | 1.705E-04                        | 1.644E-04           | 1.883E-04                        | 3.589E-04           | 2.714E-04 |
| LSDA       | 5.518E-05                        | 2.105E-04                        | 2.006E-04           | 2.389E-04                        | 4.278E-04           | 3.275E-04 |
| M06        | 2.505E-04                        | 4.617E-04                        | 4.620E-04           | 3.593E-04                        | 5.547E-04           | 3.692E-04 |
| M06-2X     | 3.155E-04                        | 5.478E-04                        | 5.111E-04           | 4.336E-04                        | 6.410E-04           | 4.331E-04 |
| MN12-SX    | 3.236E-04                        | 6.291E-04                        | 6.400E-04           | 5.292E-04                        | 8.143E-04           | 5.901E-04 |
| PBEP86     | 5.904E-05                        | 2.279E-04                        | 2.230E-04           | 2.580E-04                        | 4.758E-04           | 4.080E-04 |

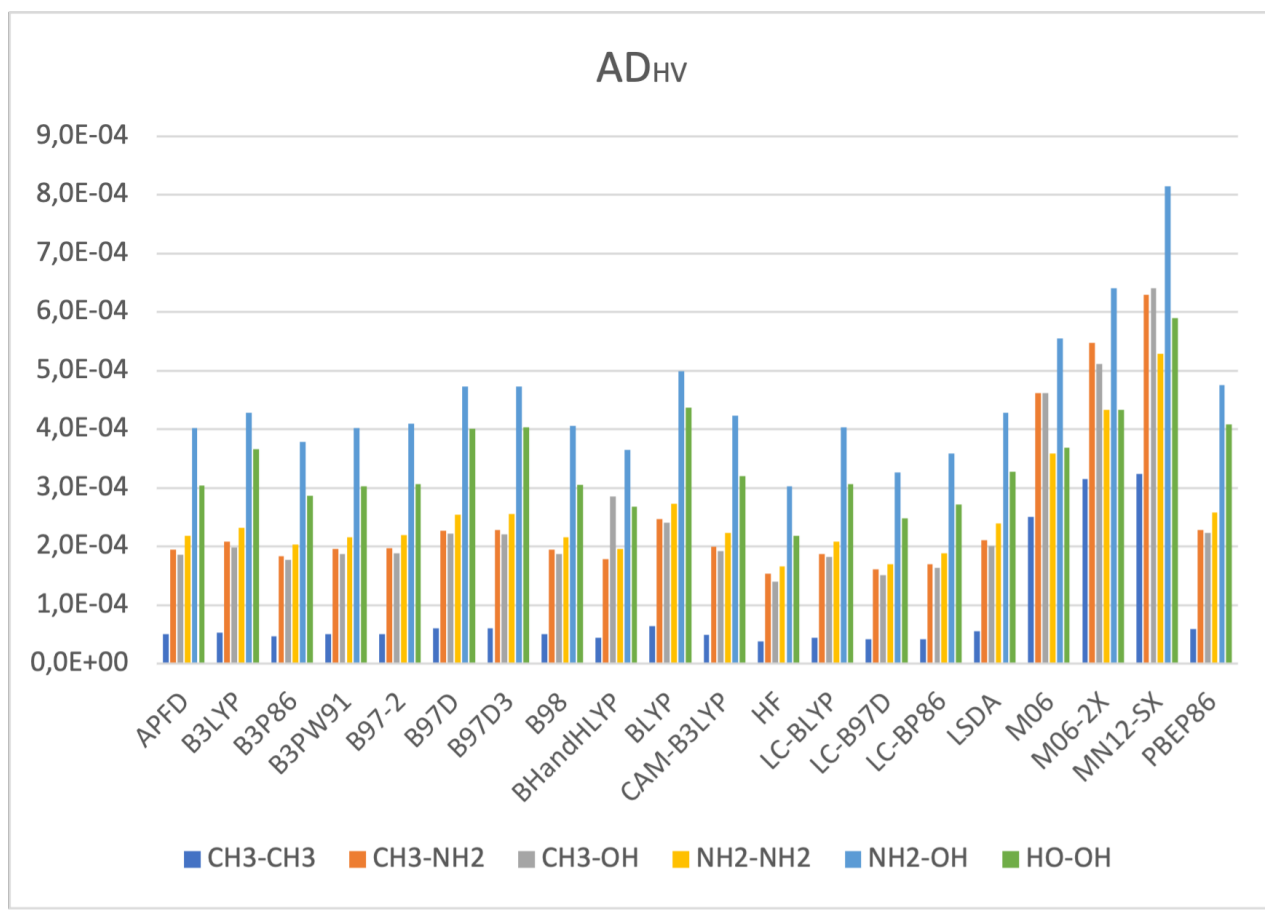

Figure S1: Histogram chart of data in Table S21.

Table S22: AD<sub>RR</sub>

| Functional | CH <sub>3</sub> -CH <sub>3</sub> | CH <sub>3</sub> -NH <sub>2</sub> | CH <sub>3</sub> -OH | NH <sub>2</sub> -NH <sub>2</sub> | NH <sub>2</sub> -OH | HO-OH     |
|------------|----------------------------------|----------------------------------|---------------------|----------------------------------|---------------------|-----------|
| APFD       | 3.438E-03                        | 3.777E-02                        | 3.411E-02           | 8.219E-02                        | 1.426E-01           | 1.187E-01 |
| B3LYP      | 4.194E-03                        | 4.387E-02                        | 3.893E-02           | 9.246E-02                        | 1.602E-01           | 1.888E-01 |
| B3P86      | 2.919E-03                        | 3.333E-02                        | 3.075E-02           | 7.224E-02                        | 1.270E-01           | 1.068E-01 |
| B3PW91     | 3.604E-03                        | 3.720E-02                        | 3.413E-02           | 8.051E-02                        | 1.397E-01           | 1.169E-01 |
| B97-2      | 3.968E-03                        | 3.766E-02                        | 3.469E-02           | 8.203E-02                        | 1.438E-01           | 1.202E-01 |
| B97D       | 6.713E-03                        | 4.842E-02                        | 4.584E-02           | 1.024E-01                        | 1.816E-01           | 2.230E-01 |
| B97D3      | 6.655E-03                        | 4.890E-02                        | 4.568E-02           | 1.033E-01                        | 1.814E-01           | 2.237E-01 |
| B98        | 3.465E-03                        | 3.777E-02                        | 3.459E-02           | 8.020E-02                        | 1.438E-01           | 1.209E-01 |
| BHandHLYP  | 2.239E-03                        | 3.218E-02                        | 8.711E-02           | 6.913E-02                        | 1.199E-01           | 9.638E-02 |
| BLYP       | 6.941E-03                        | 5.752E-02                        | 5.264E-02           | 1.187E-01                        | 2.066E-01           | 2.610E-01 |
| CAM-B3LYP  | 3.391E-03                        | 4.110E-02                        | 3.703E-02           | 8.719E-02                        | 1.554E-01           | 1.311E-01 |
| HF         | 1.419E-03                        | 2.257E-02                        | 1.991E-02           | 4.834E-02                        | 8.280E-02           | 6.311E-02 |
| LC-BLYP    | 2.191E-03                        | 3.704E-02                        | 3.323E-02           | 7.791E-02                        | 1.437E-01           | 1.216E-01 |
| LC-B97D    | 2.185E-03                        | 2.705E-02                        | 2.379E-02           | 5.301E-02                        | 1.007E-01           | 8.599E-02 |
| LC-BP86    | 1.798E-03                        | 2.927E-02                        | 2.716E-02           | 6.239E-02                        | 1.159E-01           | 9.841E-02 |
| LSDA       | 5.099E-03                        | 5.013E-02                        | 4.124E-02           | 1.085E-01                        | 1.765E-01           | 1.467E-01 |
| M06        | 7.943E-01                        | 6.924E-01                        | 5.755E-01           | 5.467E-01                        | 4.084E-01           | 2.785E-01 |
| M06-2X     | 1.722E+00                        | 1.622E+00                        | 1.486E+00           | 1.532E+00                        | 1.383E+00           | 1.230E+00 |
| MN12-SX    | 1.062E+00                        | 1.338E+00                        | 1.526E+00           | 1.598E+00                        | 1.819E+00           | 1.970E+00 |
| PBEP86     | 5.698E-03                        | 5.106E-02                        | 4.660E-02           | 1.090E-01                        | 1.909E-01           | 2.352E-01 |

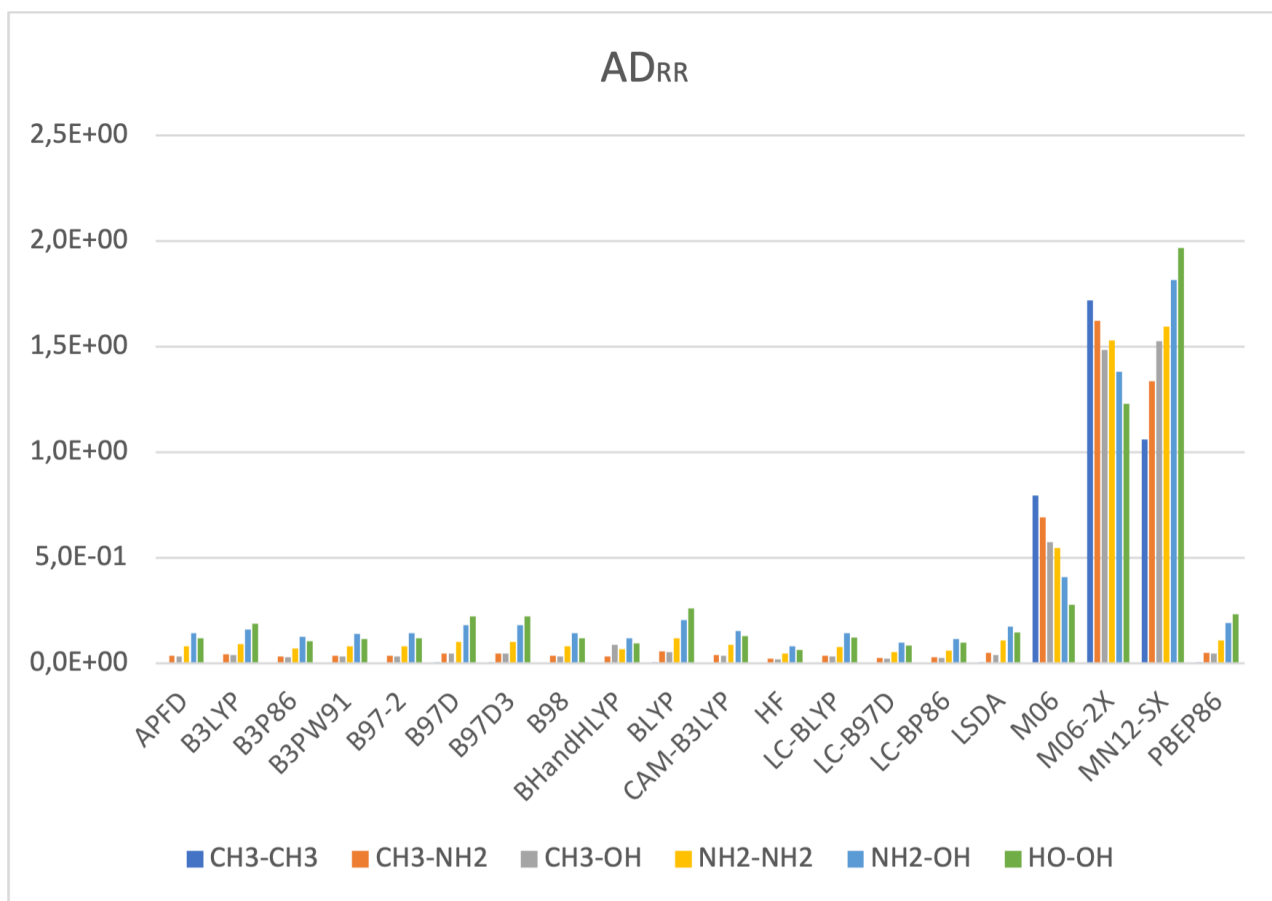

Figure S2: Histogram chart of data in Table S22.

Table S23: AD<sub>PR</sub>

| Functional | CH <sub>3</sub> -CH <sub>3</sub> | CH <sub>3</sub> -NH <sub>2</sub> | CH <sub>3</sub> -OH | NH <sub>2</sub> -NH <sub>2</sub> | NH <sub>2</sub> -OH | HO-OH     |
|------------|----------------------------------|----------------------------------|---------------------|----------------------------------|---------------------|-----------|
| APFD       | 3.206E-03                        | 5.843E-03                        | 5.296E-03           | 9.214E-03                        | 1.236E-02           | 1.474E-02 |
| B3LYP      | 3.324E-03                        | 6.368E-03                        | 5.776E-03           | 1.013E-02                        | 1.358E-02           | 1.532E-02 |
| B3P86      | 3.091E-03                        | 5.415E-03                        | 4.944E-03           | 8.401E-03                        | 1.119E-02           | 1.330E-02 |
| B3PW91     | 3.207E-03                        | 5.810E-03                        | 5.282E-03           | 9.134E-03                        | 1.214E-02           | 1.447E-02 |
| B97-2      | 2.965E-03                        | 5.708E-03                        | 5.193E-03           | 9.241E-03                        | 1.247E-02           | 1.492E-02 |
| B97D       | 3.129E-03                        | 6.747E-03                        | 6.215E-03           | 1.140E-02                        | 1.514E-02           | 1.738E-02 |
| B97D3      | 3.126E-03                        | 6.775E-03                        | 6.195E-03           | 1.142E-02                        | 1.512E-02           | 1.751E-02 |
| B98        | 3.215E-03                        | 5.890E-03                        | 5.355E-03           | 9.253E-03                        | 1.247E-02           | 1.507E-02 |
| BHandHLYP  | 2.945E-03                        | 5.120E-03                        | 8.358E-03           | 7.802E-03                        | 1.069E-02           | 1.227E-02 |
| BLYP       | 3.799E-03                        | 7.867E-03                        | 7.238E-03           | 1.287E-02                        | 1.682E-02           | 1.996E-02 |
| CAM-B3LYP  | 3.228E-03                        | 6.011E-03                        | 5.601E-03           | 9.476E-03                        | 1.327E-02           | 1.625E-02 |
| HF         | 2.594E-03                        | 4.074E-03                        | 3.686E-03           | 5.821E-03                        | 7.872E-03           | 8.332E-03 |
| LC-BLYP    | 3.145E-03                        | 5.517E-03                        | 5.297E-03           | 8.412E-03                        | 1.248E-02           | 1.526E-02 |
| LC-B97D    | 2.751E-03                        | 4.302E-03                        | 4.222E-03           | 6.186E-03                        | 9.030E-03           | 1.098E-02 |
| LC-BP86    | 3.006E-03                        | 4.866E-03                        | 4.664E-03           | 7.216E-03                        | 1.045E-02           | 1.239E-02 |
| LSDA       | 3.378E-03                        | 6.788E-03                        | 5.927E-03           | 1.123E-02                        | 1.475E-02           | 1.776E-02 |
| M06        | 4.331E-03                        | 6.676E-03                        | 6.733E-03           | 1.017E-02                        | 1.333E-02           | 1.567E-02 |
| M06-2X     | 3.202E-03                        | 6.863E-03                        | 5.432E-03           | 1.098E-02                        | 1.288E-02           | 1.491E-02 |
| MN12-SX    | 1.232E-03                        | 6.732E-03                        | 3.597E-03           | 1.562E-02                        | 1.493E-02           | 1.410E-02 |
| PBEP86     | 3.623E-03                        | 7.247E-03                        | 6.634E-03           | 1.191E-02                        | 1.570E-02           | 1.830E-02 |

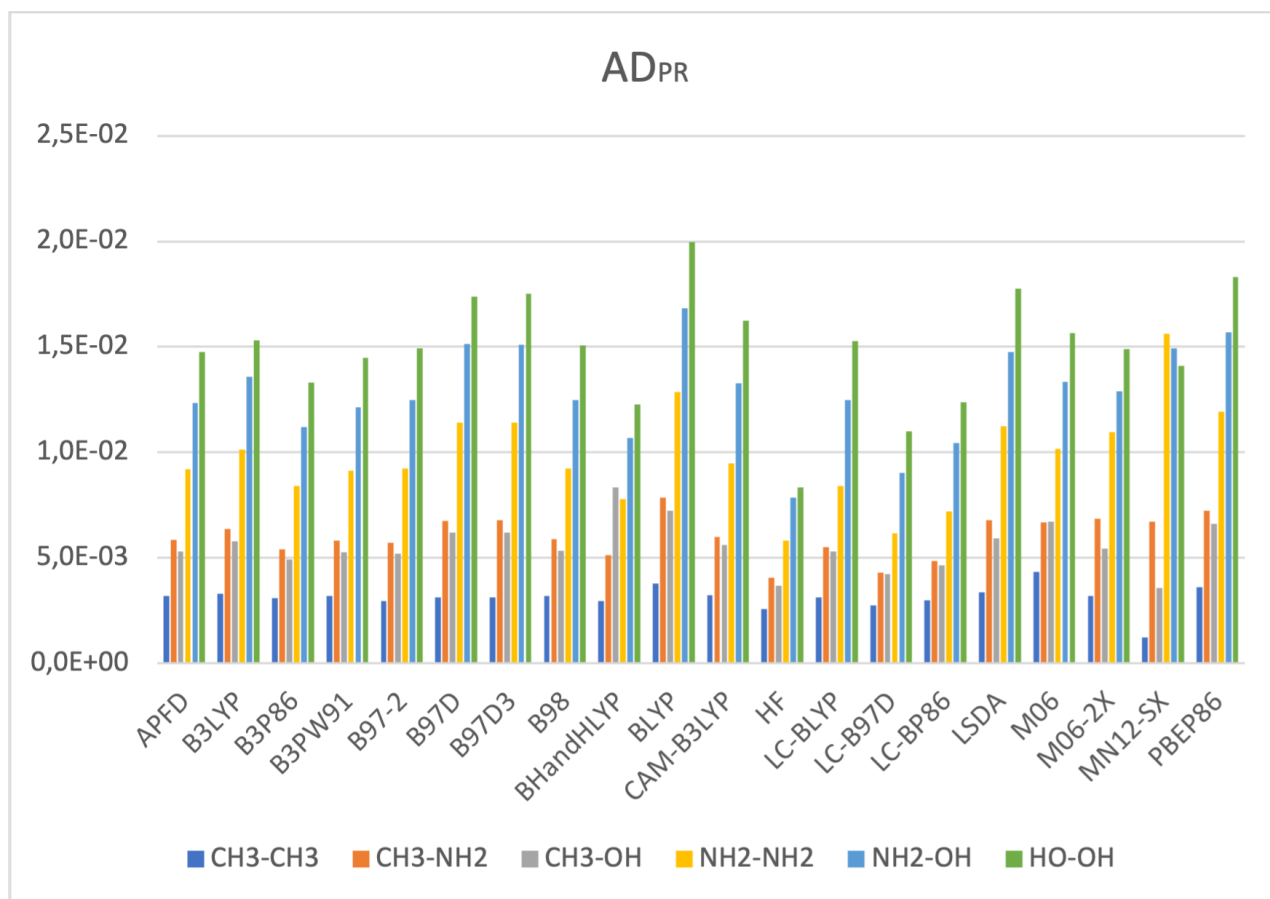

Figure S3: Histogram chart of data in Table S23.

Table S24: AD<sub>PP</sub>

| Functional | CH <sub>3</sub> -CH <sub>3</sub> | CH <sub>3</sub> -NH <sub>2</sub> | CH <sub>3</sub> -OH | NH <sub>2</sub> -NH <sub>2</sub> | NH <sub>2</sub> -OH | HO-OH     |
|------------|----------------------------------|----------------------------------|---------------------|----------------------------------|---------------------|-----------|
| APFD       | 6.791E-03                        | 1.976E-02                        | 1.974E-02           | 4.086E-02                        | 5.870E-02           | 7.022E-02 |
| B3LYP      | 7.415E-03                        | 2.208E-02                        | 2.196E-02           | 4.542E-02                        | 6.476E-02           | 7.737E-02 |
| B3P86      | 6.386E-03                        | 1.819E-02                        | 1.833E-02           | 3.713E-02                        | 5.345E-02           | 6.429E-02 |
| B3PW91     | 6.883E-03                        | 1.966E-02                        | 1.973E-02           | 4.030E-02                        | 5.757E-02           | 6.911E-02 |
| B97-2      | 6.799E-03                        | 1.967E-02                        | 1.981E-02           | 4.083E-02                        | 5.882E-02           | 7.058E-02 |
| B97D       | 8.570E-03                        | 2.422E-02                        | 2.437E-02           | 5.008E-02                        | 7.040E-02           | 8.603E-02 |
| B97D3      | 8.535E-03                        | 2.432E-02                        | 2.428E-02           | 5.023E-02                        | 7.030E-02           | 8.650E-02 |
| B98        | 6.777E-03                        | 1.990E-02                        | 2.000E-02           | 4.073E-02                        | 5.920E-02           | 7.149E-02 |
| BHandHLYP  | 5.779E-03                        | 1.731E-02                        | 3.630E-02           | 3.520E-02                        | 5.177E-02           | 5.966E-02 |
| BLYP       | 9.544E-03                        | 2.784E-02                        | 2.754E-02           | 5.690E-02                        | 7.889E-02           | 9.889E-02 |
| CAM-B3LYP  | 6.869E-03                        | 2.098E-02                        | 2.142E-02           | 4.294E-02                        | 6.370E-02           | 7.730E-02 |
| HF         | 4.793E-03                        | 1.368E-02                        | 1.352E-02           | 2.619E-02                        | 3.877E-02           | 4.192E-02 |
| LC-BLYP    | 6.078E-03                        | 1.913E-02                        | 2.008E-02           | 3.847E-02                        | 6.041E-02           | 7.315E-02 |
| LC-B97D    | 5.572E-03                        | 1.507E-02                        | 1.599E-02           | 2.892E-02                        | 4.581E-02           | 5.571E-02 |
| LC-BP86    | 5.651E-03                        | 1.618E-02                        | 1.723E-02           | 3.230E-02                        | 5.059E-02           | 6.077E-02 |
| LSDA       | 8.042E-03                        | 2.422E-02                        | 2.269E-02           | 5.077E-02                        | 6.990E-02           | 8.365E-02 |
| M06        | 8.549E-01                        | 7.651E-01                        | 6.409E-01           | 6.129E-01                        | 4.782E-01           | 3.354E-01 |
| M06-2X     | 1.800E+00                        | 1.706E+00                        | 1.552E+00           | 1.617E+00                        | 1.467E+00           | 1.309E+00 |
| MN12-SX    | 9.490E-01                        | 1.200E+00                        | 1.375E+00           | 1.425E+00                        | 1.609E+00           | 1.792E+00 |
| PBEP86     | 8.661E-03                        | 2.535E-02                        | 2.497E-02           | 5.282E-02                        | 7.394E-02           | 9.115E-02 |

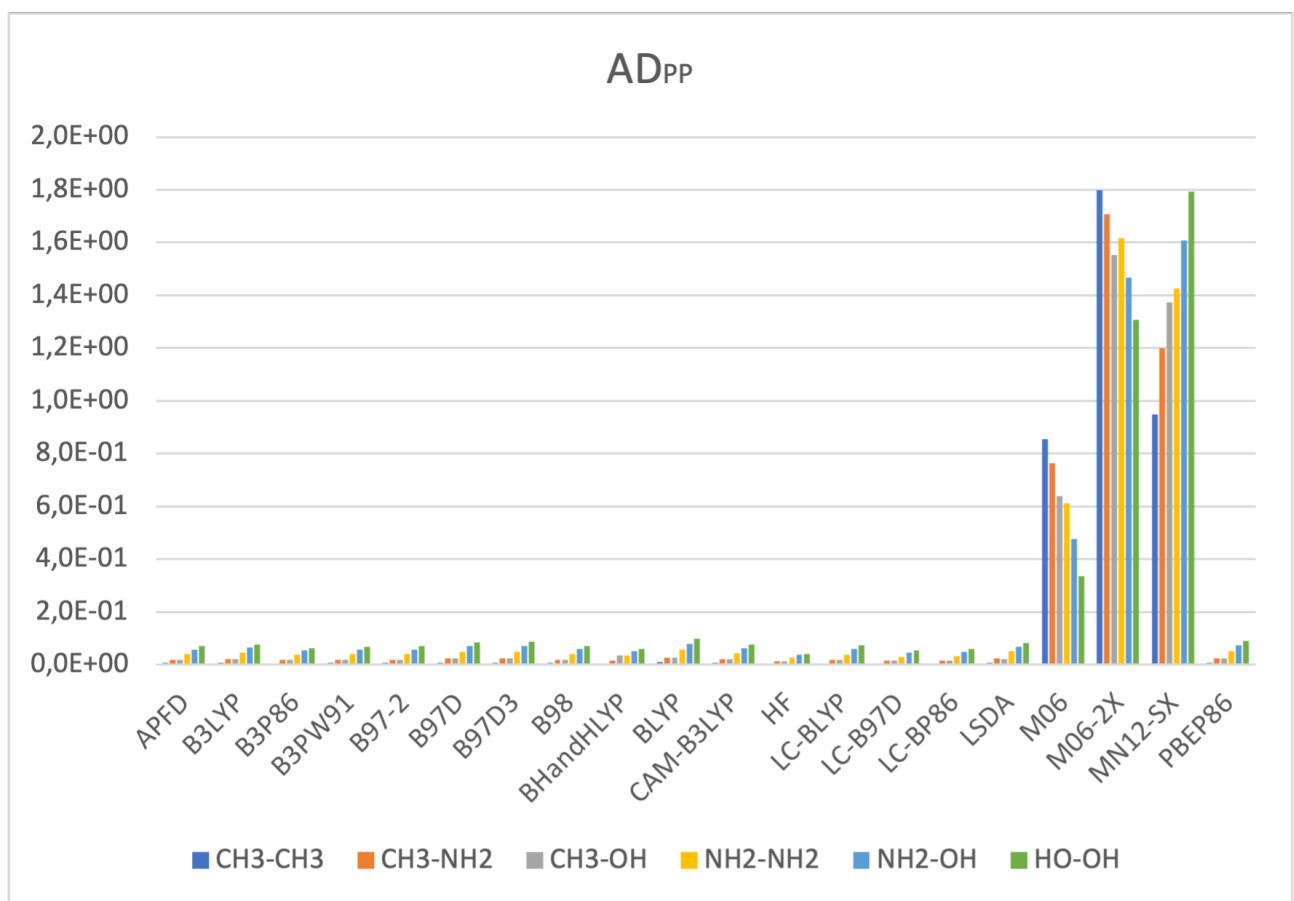

Figure S4: Histogram chart of data in Table S24.

Table S25: AD<sub>RL</sub>

| Functional | CH <sub>3</sub> -CH <sub>3</sub> | CH <sub>3</sub> -NH <sub>2</sub> | CH <sub>3</sub> -OH | NH <sub>2</sub> -NH <sub>2</sub> | NH <sub>2</sub> -OH | HO-OH     |
|------------|----------------------------------|----------------------------------|---------------------|----------------------------------|---------------------|-----------|
| APFD       | 3.337E-04                        | 2.898E-03                        | 2.266E-03           | 6.740E-03                        | 5.071E-03           | 7.471E-03 |
| B3LYP      | 3.720E-04                        | 3.350E-03                        | 2.721E-03           | 7.541E-03                        | 5.887E-03           | 6.714E-03 |
| B3P86      | 2.914E-04                        | 2.563E-03                        | 2.075E-03           | 5.933E-03                        | 4.501E-03           | 6.717E-03 |
| B3PW91     | 3.653E-04                        | 2.824E-03                        | 2.232E-03           | 6.653E-03                        | 4.991E-03           | 7.352E-03 |
| B97-2      | 3.281E-04                        | 2.997E-03                        | 2.458E-03           | 6.741E-03                        | 5.175E-03           | 7.544E-03 |
| B97D       | 4.663E-04                        | 4.002E-03                        | 3.366E-03           | 8.951E-03                        | 6.786E-03           | 7.551E-03 |
| B97D3      | 4.478E-04                        | 4.049E-03                        | 3.390E-03           | 8.999E-03                        | 6.809E-03           | 7.624E-03 |
| B98        | 3.258E-04                        | 3.038E-03                        | 2.454E-03           | 6.602E-03                        | 5.292E-03           | 7.622E-03 |
| BHandHLYP  | 2.460E-04                        | 2.417E-03                        | 2.499E-03           | 5.224E-03                        | 4.184E-03           | 6.128E-03 |
| BLYP       | 5.386E-04                        | 4.570E-03                        | 3.916E-03           | 1.035E-02                        | 8.036E-03           | 8.687E-03 |
| CAM-B3LYP  | 3.406E-04                        | 3.082E-03                        | 2.687E-03           | 6.692E-03                        | 5.772E-03           | 8.286E-03 |
| HF         | 1.702E-04                        | 1.662E-03                        | 1.224E-03           | 3.371E-03                        | 2.800E-03           | 3.994E-03 |
| LC-BLYP    | 2.529E-04                        | 2.647E-03                        | 2.408E-03           | 5.479E-03                        | 5.494E-03           | 7.722E-03 |
| LC-B97D    | 1.246E-04                        | 1.873E-03                        | 1.785E-03           | 3.591E-03                        | 4.043E-03           | 5.458E-03 |
| LC-BP86    | 2.205E-04                        | 2.056E-03                        | 1.769E-03           | 4.447E-03                        | 4.287E-03           | 6.180E-03 |
| LSDA       | 4.379E-04                        | 3.634E-03                        | 2.723E-03           | 9.026E-03                        | 6.606E-03           | 9.199E-03 |
| M06        | 5.363E-04                        | 3.469E-03                        | 2.310E-03           | 9.045E-03                        | 6.949E-03           | 8.191E-03 |
| M06-2X     | 3.436E-04                        | 3.898E-03                        | 2.328E-03           | 5.532E-03                        | 4.172E-03           | 6.923E-03 |
| MN12-SX    | 7.544E-04                        | 7.431E-03                        | 3.551E-03           | 1.145E-02                        | 8.086E-03           | 9.034E-03 |
| PBEP86     | 4.874E-04                        | 4.094E-03                        | 3.304E-03           | 9.418E-03                        | 7.247E-03           | 7.995E-03 |

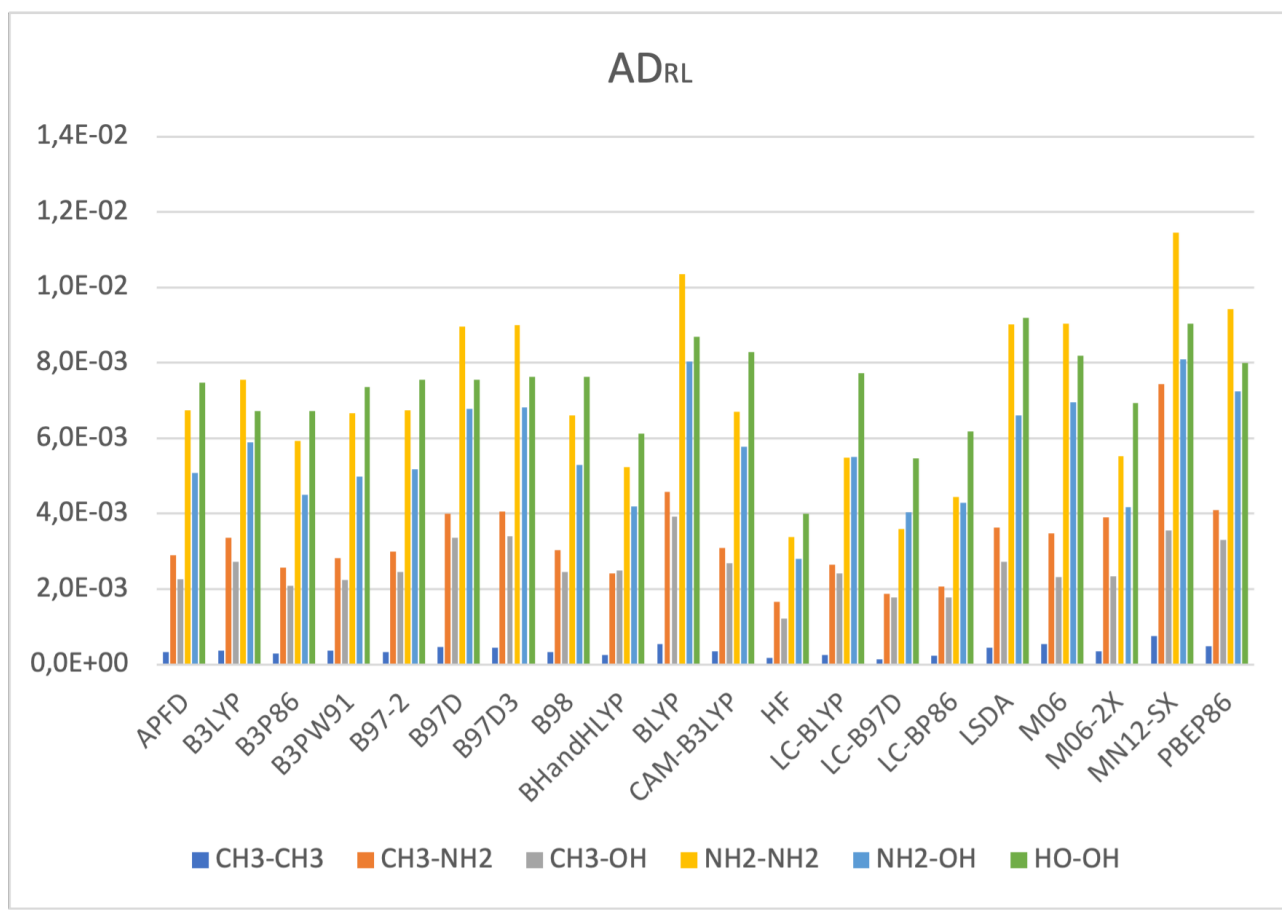

Figure S5: Histogram chart of data in Table S25.

Table S26: AD<sub>PL</sub>

| Functional | CH <sub>3</sub> -CH <sub>3</sub> | CH <sub>3</sub> -NH <sub>2</sub> | CH <sub>3</sub> -OH | NH <sub>2</sub> -NH <sub>2</sub> | NH <sub>2</sub> -OH | HO-OH     |
|------------|----------------------------------|----------------------------------|---------------------|----------------------------------|---------------------|-----------|
| APFD       | 2.064E-03                        | 1.857E-02                        | 1.406E-02           | 5.163E-02                        | 4.285E-02           | 3.768E-02 |
| B3LYP      | 2.262E-03                        | 2.111E-02                        | 1.638E-02           | 5.732E-02                        | 4.686E-02           | 4.055E-02 |
| B3P86      | 1.813E-03                        | 1.668E-02                        | 1.289E-02           | 4.530E-02                        | 3.726E-02           | 3.378E-02 |
| B3PW91     | 2.097E-03                        | 1.794E-02                        | 1.376E-02           | 5.024E-02                        | 4.161E-02           | 3.673E-02 |
| B97-2      | 2.025E-03                        | 1.843E-02                        | 1.423E-02           | 5.174E-02                        | 4.328E-02           | 3.766E-02 |
| B97D       | 2.687E-03                        | 2.276E-02                        | 1.763E-02           | 6.544E-02                        | 5.407E-02           | 4.446E-02 |
| B97D3      | 2.670E-03                        | 2.278E-02                        | 1.754E-02           | 6.582E-02                        | 5.401E-02           | 4.459E-02 |
| B98        | 2.004E-03                        | 1.917E-02                        | 1.477E-02           | 5.083E-02                        | 4.220E-02           | 3.839E-02 |
| BHandHLYP  | 1.545E-03                        | 1.666E-02                        | 2.487E-02           | 4.238E-02                        | 3.528E-02           | 3.240E-02 |
| BLYP       | 3.159E-03                        | 2.622E-02                        | 2.068E-02           | 7.458E-02                        | 5.978E-02           | 5.162E-02 |
| CAM-B3LYP  | 1.980E-03                        | 2.061E-02                        | 1.650E-02           | 5.339E-02                        | 4.527E-02           | 4.240E-02 |
| HF         | 1.048E-03                        | 1.251E-02                        | 9.422E-03           | 2.947E-02                        | 2.486E-02           | 2.275E-02 |
| LC-BLYP    | 1.556E-03                        | 1.909E-02                        | 1.598E-02           | 4.666E-02                        | 4.452E-02           | 4.074E-02 |
| LC-B97D    | 1.003E-03                        | 1.435E-02                        | 1.241E-02           | 3.190E-02                        | 3.411E-02           | 3.009E-02 |
| LC-BP86    | 1.377E-03                        | 1.531E-02                        | 1.260E-02           | 3.797E-02                        | 3.539E-02           | 3.290E-02 |
| LSDA       | 2.734E-03                        | 2.277E-02                        | 1.582E-02           | 6.893E-02                        | 5.581E-02           | 4.592E-02 |
| M06        | 8.575E-03                        | 1.845E-01                        | 3.420E-01           | 4.667E-02                        | 1.886E-01           | 3.429E-02 |
| M06-2X     | 1.310E-03                        | 6.541E-02                        | 1.529E-01           | 7.343E-02                        | 1.513E-01           | 5.439E-02 |
| MN12-SX    | 1.798E-02                        | 3.191E-01                        | 5.125E-01           | 1.336E-01                        | 2.721E-01           | 9.613E-02 |
| PBEP86     | 2.918E-03                        | 2.410E-02                        | 1.832E-02           | 7.063E-02                        | 5.708E-02           | 4.756E-02 |

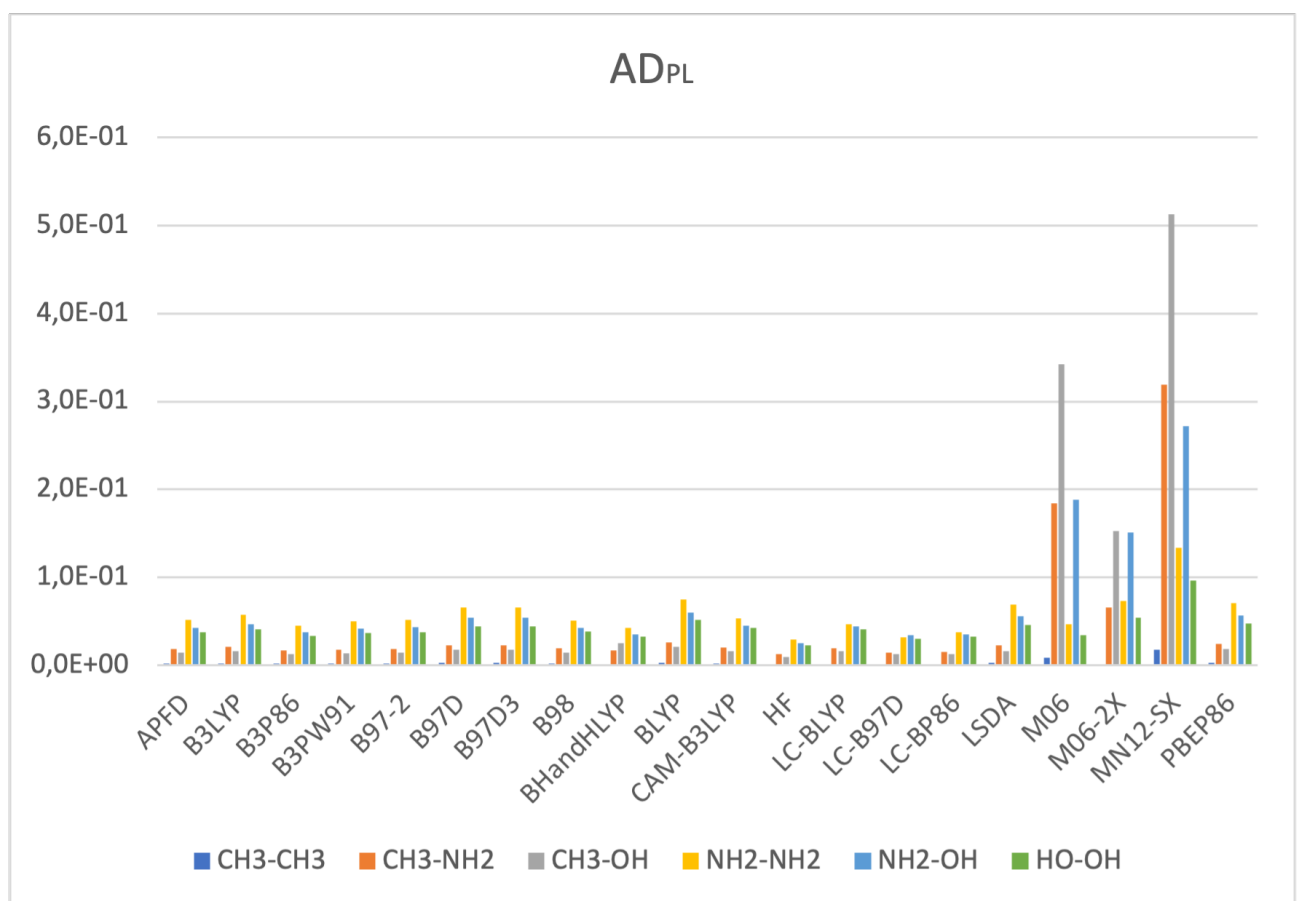

Figure S6: Histogram chart of data in Table S26.

Table S27:  $AD_\alpha$ 

| Functional | CH <sub>3</sub> -CH <sub>3</sub> | CH <sub>3</sub> -NH <sub>2</sub> | CH <sub>3</sub> -OH | NH <sub>2</sub> -NH <sub>2</sub> | NH <sub>2</sub> -OH | HO-OH     |
|------------|----------------------------------|----------------------------------|---------------------|----------------------------------|---------------------|-----------|
| APFD       | 1.562E-01                        | 4.887E-01                        | 3.267E-01           | 9.259E-01                        | 9.056E-01           | 8.811E-01 |
| B3LYP      | 1.746E-01                        | 5.503E-01                        | 3.654E-01           | 1.028E+00                        | 9.870E-01           | 9.802E-01 |
| B3P86      | 1.429E-01                        | 4.520E-01                        | 2.982E-01           | 8.704E-01                        | 8.464E-01           | 8.306E-01 |
| B3PW91     | 1.581E-01                        | 4.873E-01                        | 3.253E-01           | 9.174E-01                        | 8.910E-01           | 8.708E-01 |
| B97-2      | 1.556E-01                        | 4.861E-01                        | 3.277E-01           | 9.215E-01                        | 9.080E-01           | 8.848E-01 |
| B97D       | 2.126E-01                        | 6.332E-01                        | 4.248E-01           | 1.150E+00                        | 1.099E+00           | 1.089E+00 |
| B97D3      | 2.115E-01                        | 6.346E-01                        | 4.233E-01           | 1.155E+00                        | 1.098E+00           | 1.094E+00 |
| B98        | 1.535E-01                        | 4.917E-01                        | 3.309E-01           | 9.283E-01                        | 9.145E-01           | 9.011E-01 |
| BHandHLYP  | 1.189E-01                        | 4.026E-01                        | 8.015E-01           | 7.732E-01                        | 7.699E-01           | 7.400E-01 |
| BLYP       | 2.436E-01                        | 7.138E-01                        | 4.829E-01           | 1.286E+00                        | 1.188E+00           | 1.206E+00 |
| CAM-B3LYP  | 1.550E-01                        | 5.081E-01                        | 3.492E-01           | 9.532E-01                        | 9.599E-01           | 9.699E-01 |
| HF         | 8.470E-02                        | 2.887E-01                        | 2.031E-01           | 5.481E-01                        | 5.599E-01           | 5.114E-01 |
| LC-BLYP    | 1.230E-01                        | 4.476E-01                        | 3.261E-01           | 8.387E-01                        | 8.963E-01           | 9.261E-01 |
| LC-B97D    | 7.834E-02                        | 3.502E-01                        | 2.497E-01           | 6.495E-01                        | 7.125E-01           | 7.533E-01 |
| LC-BP86    | 1.086E-01                        | 3.774E-01                        | 2.705E-01           | 7.181E-01                        | 7.718E-01           | 7.950E-01 |
| LSDA       | 2.016E-01                        | 6.393E-01                        | 4.057E-01           | 1.221E+00                        | 1.138E+00           | 1.066E+00 |
| M06        | 1.003E+00                        | 8.748E+00                        | 6.703E+00           | 6.512E+00                        | 4.832E+00           | 2.605E+00 |
| M06-2X     | 1.345E+00                        | 1.147E+00                        | 8.944E+00           | 9.625E+00                        | 7.534E+00           | 5.478E+00 |
| MN12-SX    | 1.253E+00                        | 1.045E+00                        | 1.135E+00           | 2.396E+00                        | 2.999E+00           | 4.207E+00 |
| PBEP86     | 2.232E-01                        | 6.625E-01                        | 4.450E-01           | 1.229E+00                        | 1.158E+00           | 1.150E+00 |

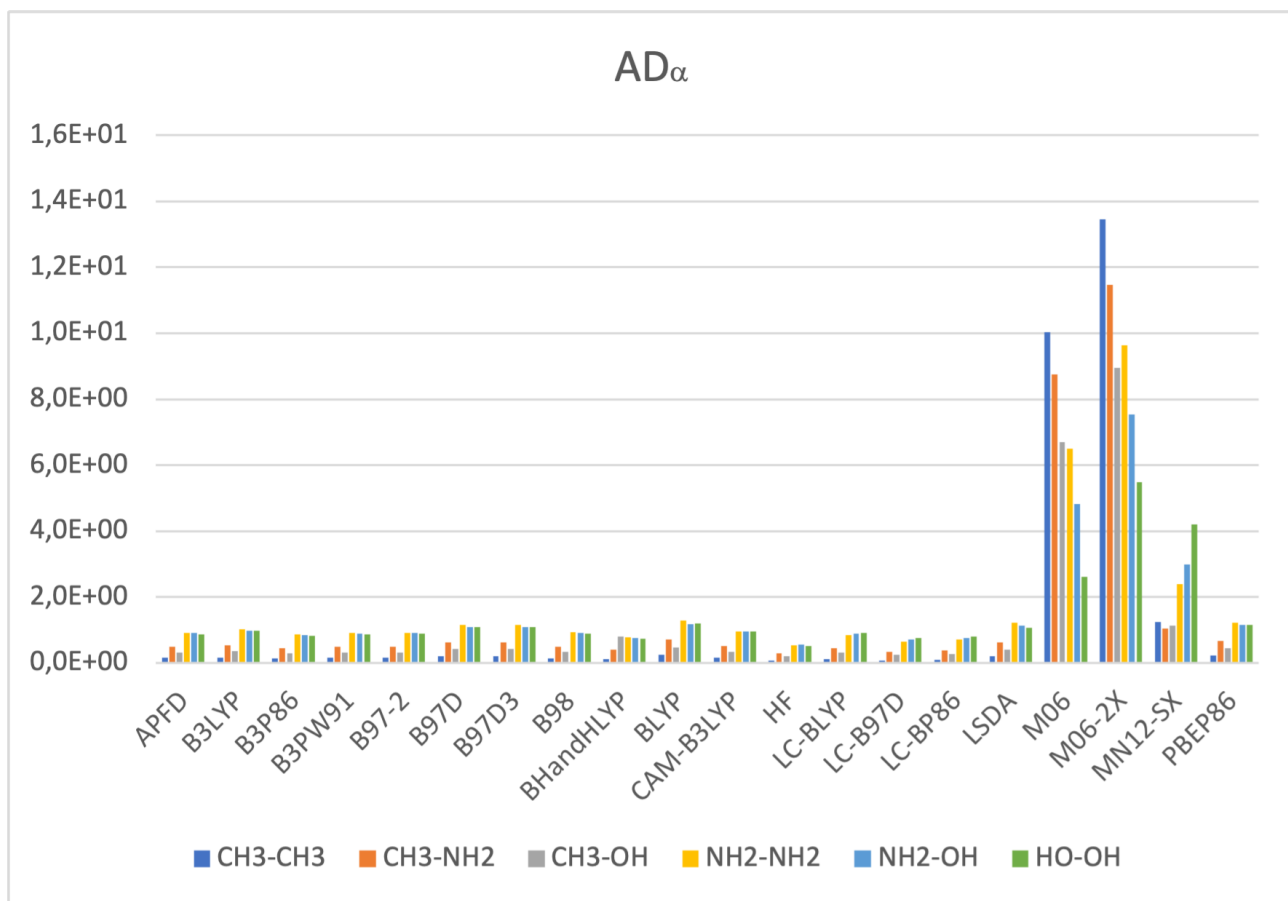

Figure S7: Histogram chart of data in Table S27.

Table S28:  $AD_{\hat{\kappa}}$ 

| Functional | CH <sub>3</sub> -CH <sub>3</sub> | CH <sub>3</sub> -NH <sub>2</sub> | CH <sub>3</sub> -OH | NH <sub>2</sub> -NH <sub>2</sub> | NH <sub>2</sub> -OH | HO-OH     |
|------------|----------------------------------|----------------------------------|---------------------|----------------------------------|---------------------|-----------|
| APFD       | 8.175E-02                        | 4.381E-01                        | 3.277E-01           | 1.897E+00                        | 2.220E+00           | 8.637E-01 |
| B3LYP      | 9.206E-02                        | 5.060E-01                        | 3.718E-01           | 2.105E+00                        | 2.495E+00           | 9.512E-01 |
| B3P86      | 7.013E-02                        | 3.964E-01                        | 2.794E-01           | 1.683E+00                        | 1.940E+00           | 7.865E-01 |
| B3PW91     | 8.104E-02                        | 4.283E-01                        | 3.357E-01           | 1.797E+00                        | 2.210E+00           | 8.463E-01 |
| B97-2      | 8.061E-02                        | 4.492E-01                        | 3.325E-01           | 1.919E+00                        | 2.224E+00           | 8.673E-01 |
| B97D       | 1.129E-01                        | 7.474E-01                        | 5.770E-01           | 2.595E+00                        | 3.319E+00           | 1.122E+00 |
| B97D3      | 1.142E-01                        | 7.643E-01                        | 5.728E-01           | 2.603E+00                        | 3.315E+00           | 1.119E+00 |
| B98        | 8.001E-02                        | 4.736E-01                        | 3.194E-01           | 1.922E+00                        | 2.155E+00           | 8.831E-01 |
| BHandHLYP  | 5.823E-02                        | 4.350E-01                        | 2.927E+00           | 1.546E+00                        | 1.538E+00           | 6.959E-01 |
| BLYP       | 1.361E-01                        | 1.096E+00                        | 6.982E-01           | 3.003E+00                        | 3.932E+00           | 1.287E+00 |
| CAM-B3LYP  | 7.903E-02                        | 5.596E-01                        | 2.862E-01           | 2.060E+00                        | 2.204E+00           | 9.959E-01 |
| HF         | 3.700E-02                        | 3.620E-01                        | 1.691E-01           | 1.019E+00                        | 9.044E-01           | 4.488E-01 |
| LC-BLYP    | 5.956E-02                        | 5.800E-01                        | 3.142E-01           | 1.832E+00                        | 1.855E+00           | 9.567E-01 |
| LC-B97D    | 3.407E-02                        | 4.606E-01                        | 2.561E-01           | 1.326E+00                        | 1.228E+00           | 7.302E-01 |
| LC-BP86    | 5.083E-02                        | 4.612E-01                        | 2.320E-01           | 1.482E+00                        | 1.512E+00           | 7.830E-01 |
| LSDA       | 1.164E-01                        | 8.045E-01                        | 5.423E-01           | 2.903E+00                        | 3.489E+00           | 1.141E+00 |
| M06        | 1.526E-01                        | 3.097E+00                        | 5.595E+00           | 4.073E+00                        | 5.242E+00           | 9.658E-01 |
| M06-2X     | 2.559E-01                        | 2.130E+00                        | 4.392E+00           | 6.787E+00                        | 5.695E+00           | 2.646E+00 |
| MN12-SX    | 5.844E-01                        | 2.531E+00                        | 4.142E+00           | 2.396E+00                        | 4.865E+00           | 2.305E+00 |
| PBEP86     | 1.259E-01                        | 8.910E-01                        | 6.447E-01           | 2.981E+00                        | 3.711E+00           | 1.212E+00 |

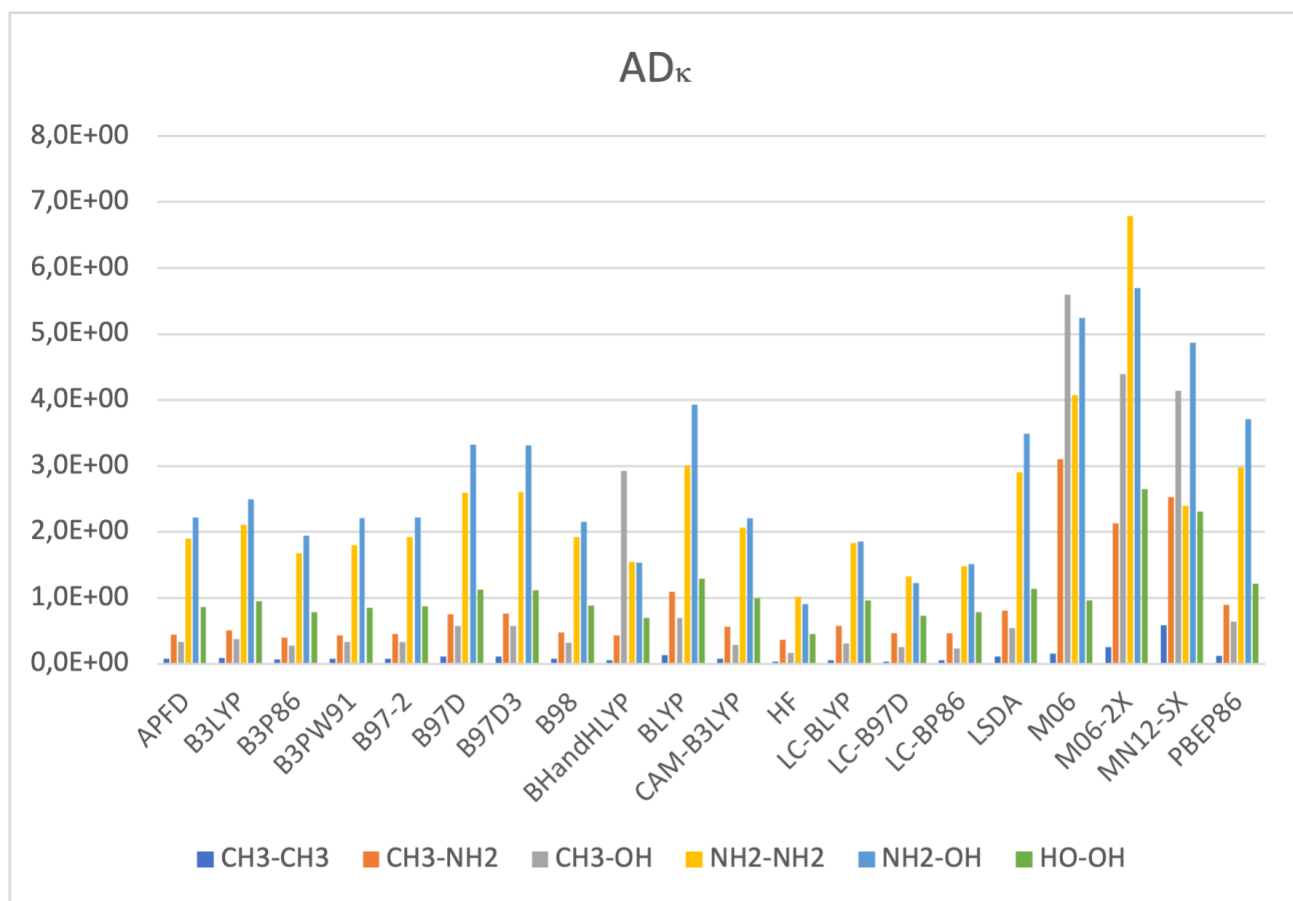

Figure S8: Histogram chart of data in Table S28.
